# Supplementary material for: Spin Hall Conductivity and Anomalous Hall Conductivity in Full Heusler compounds
Source: arXiv:2112.08630 source file (2021-12-16)
Supplement: Supplementary file 1 [file Supplemented_Materials.pdf]

# Supplemented Materials for "Spin Hall Conductivity and Anomalous Hall Conductivity in Full Heusler compounds"

Yimin Ji,[1] Wenxu Zhang,[1,*] Hongbin Zhang,[2,†] and Wanli Zhang[1]

[1] *State Key Laboratory of Electronic Thin Films and Integrated Devices, University of Electronic Science and Technology of China, Chengdu, 610054, P. R. China*

[2] *Institute of Materials Science, Technische Universtät Darmstadt, Darmstadt, 64287, Germany*

(Dated: December 13, 2021)

## I. DETAILS FOR FERROMAGNETIC FULL HEUSLER MATERIALS

The band structures of ferromagnetic full Heusler materials as well as the corresponding SHC and AHC within ±2 eV around the Fermi level are shown in the below.

### 1. $Au_2MnAl$

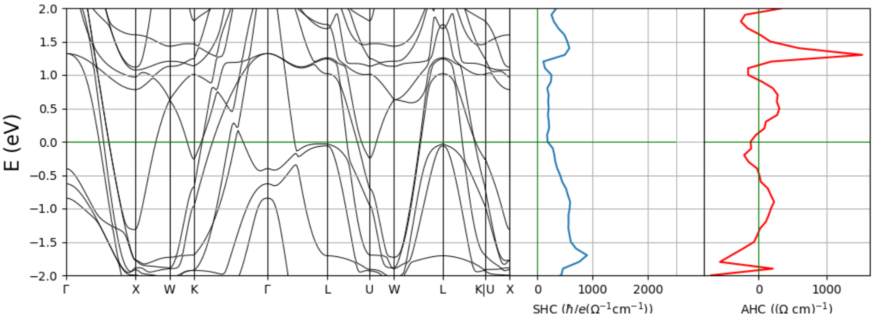


FIG. 1: The electronic band structures and corresponding SHC, AHC for $Au_2MnAl$

### 2. $Co_2NbAl$

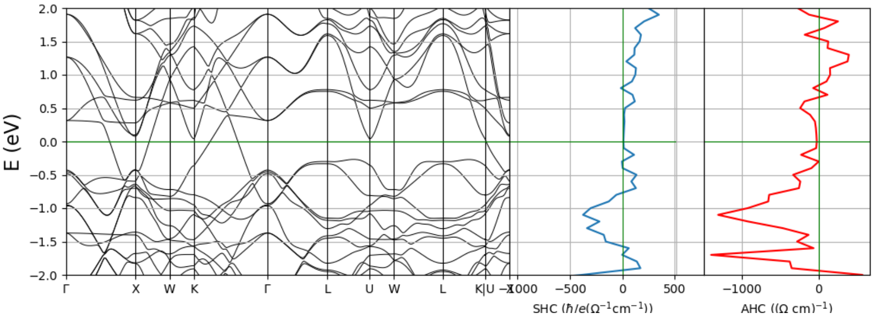


FIG. 2: The electronic band structures and corresponding SHC, AHC for $Co_2NbAl$

* xwzhang@uestc.edu.cn

† hzhang@tu-darmstadt.de

### 3. $Co_2TaAl$

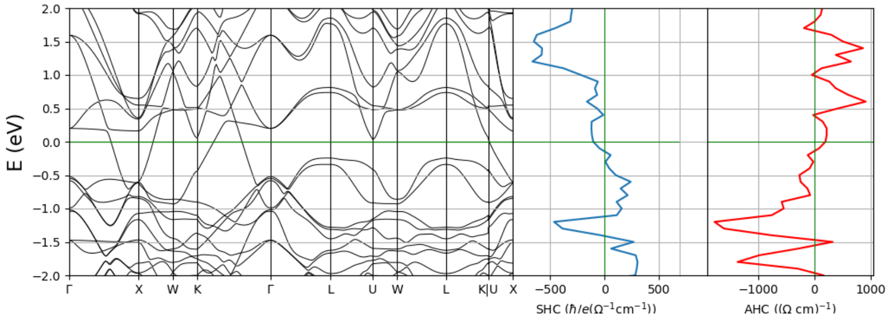


FIG. 3: The electronic band structures and corresponding SHC, AHC for $Co_2TaAl$

### 4. $Co_2CrAl$

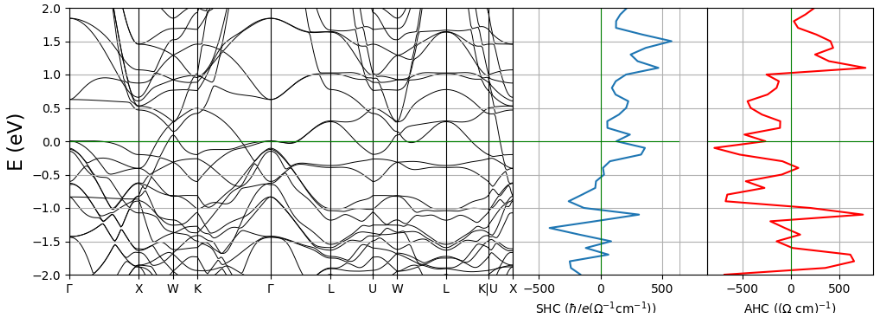


FIG. 4: The electronic band structures and corresponding SHC, AHC for $Co_2CrAl$

### 5. $Co_2CrIn$

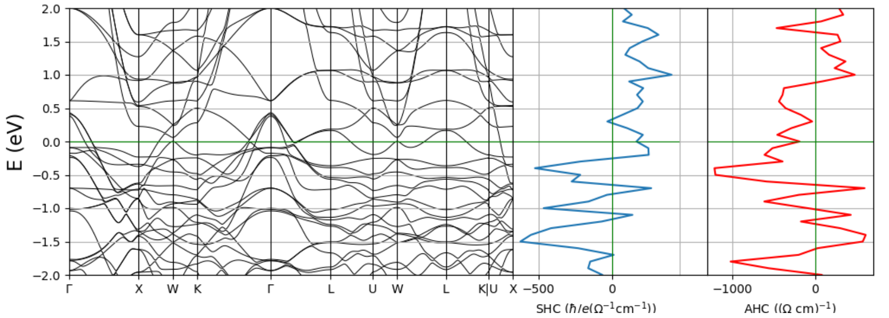


FIG. 5: The electronic band structures and corresponding SHC, AHC for $Co_2CrIn$

### 6. $Co_2FeAl$

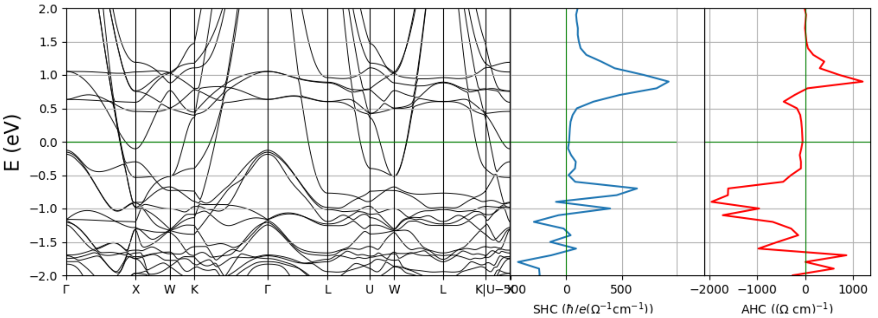


FIG. 6: The electronic band structures and corresponding SHC, AHC for $Co_2FeAl$

### 7. $Co_2CrGa$

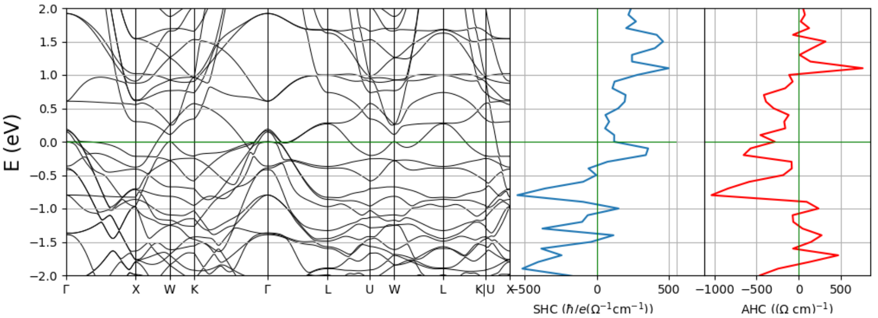


FIG. 7: The electronic band structures and corresponding SHC, AHC for $Co_2GaCr$

### 8. $Co_2FeGa$

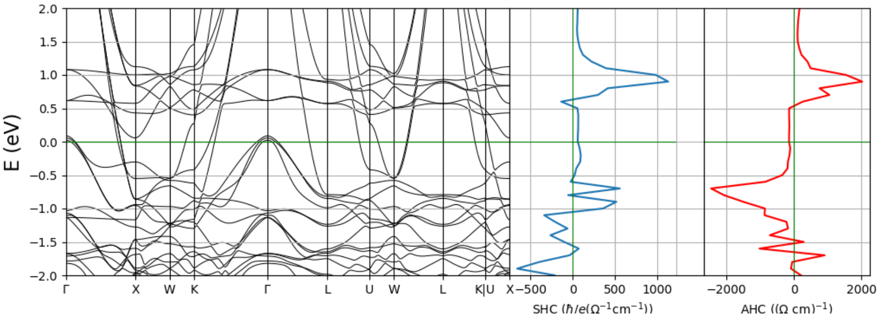


FIG. 8: The electronic band structures and corresponding SHC, AHC for $Co_2FeGa$

### 9. $Co_2MnGa$

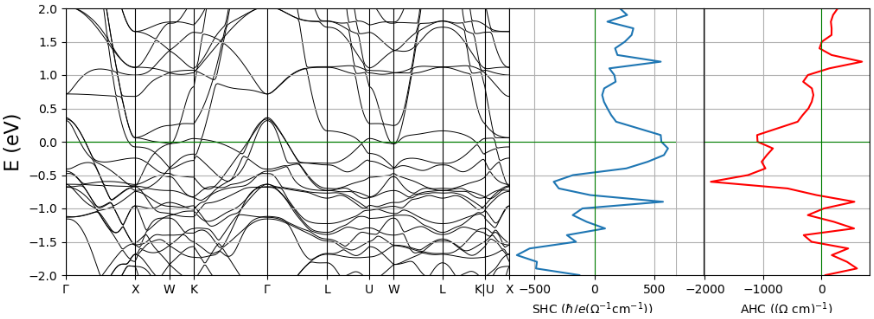


FIG. 9: The electronic band structures and corresponding SHC, AHC for $Co_2MnGa$

### 10. $Co_2FeGe$

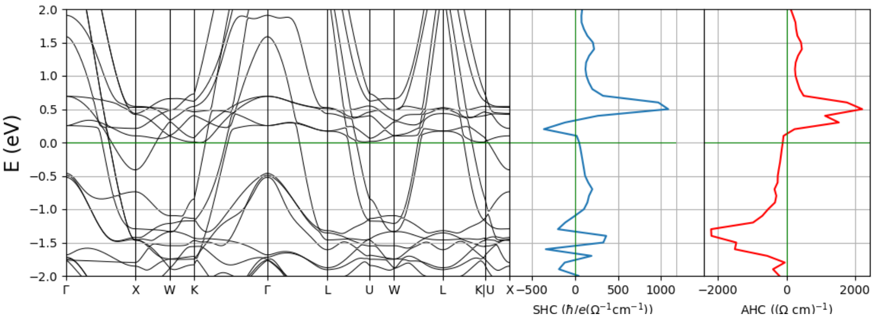


FIG. 10: The electronic band structures and corresponding SHC, AHC for $Co_2FeGe$

### 11. $Co_2HfAl$

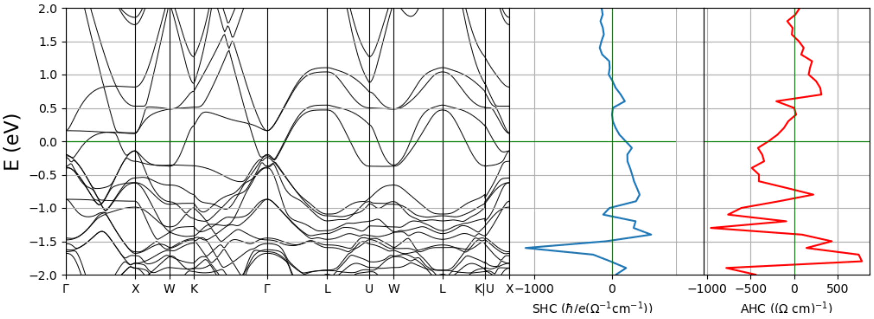


FIG. 11: The electronic band structures and corresponding SHC, AHC for $Co_2HfAl$

### 12. $Co_2HfGa$

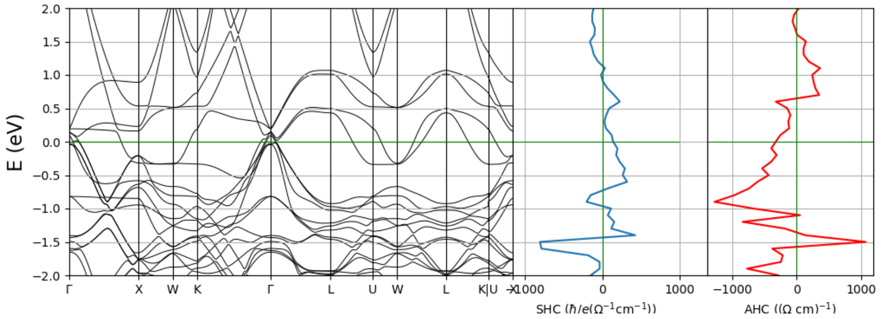


FIG. 12: The electronic band structures and corresponding SHC, AHC for $Co_2HfGa$

### 13. $Co_2HfSn$

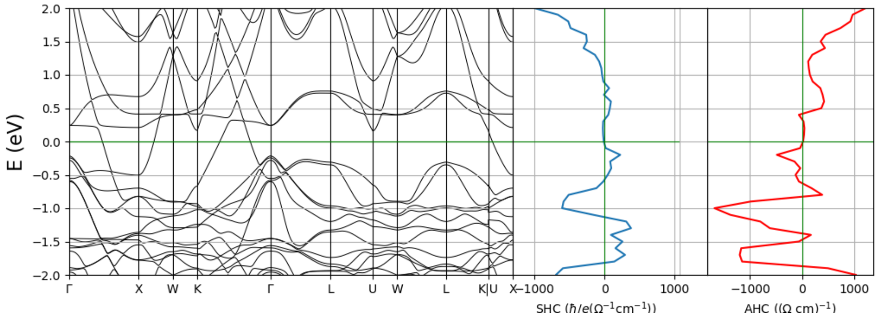


FIG. 13: The electronic band structures and corresponding SHC, AHC for $Co_2HfSn$

### 14. $Co_2FeIn$

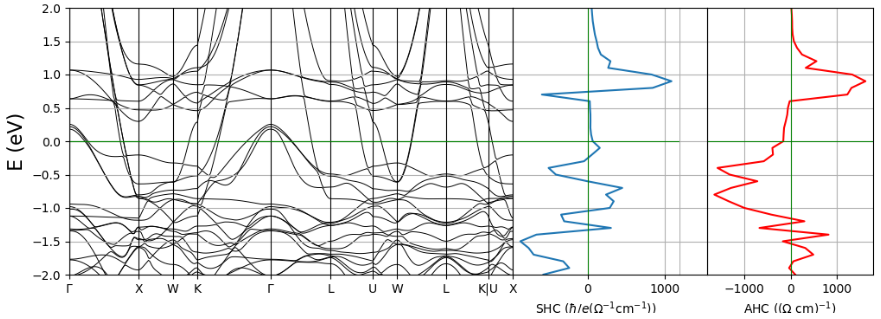


FIG. 14: The electronic band structures and corresponding SHC, AHC for $Co_2FeIn$

### 15. $Co_2MnAl$

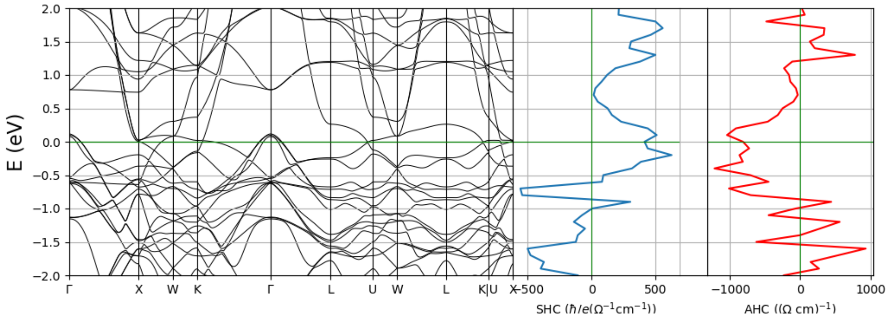


FIG. 15: The electronic band structures and corresponding SHC, AHC for $Co_2MnAl$

### 16. $Co_2MnGe$

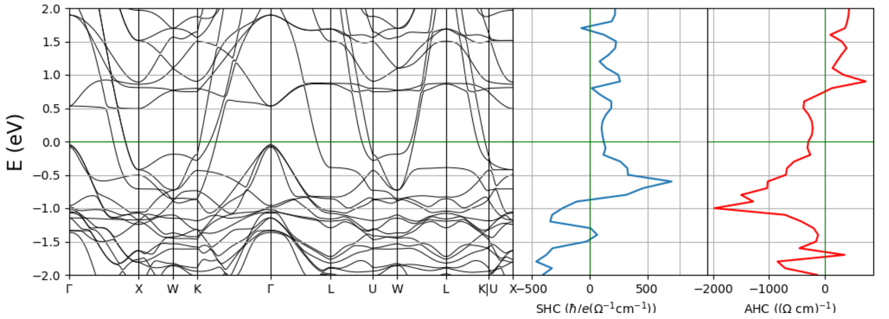


FIG. 16: The electronic band structures and corresponding SHC, AHC for $Co_2MnGe$

### 17. $Co_2NbGa$

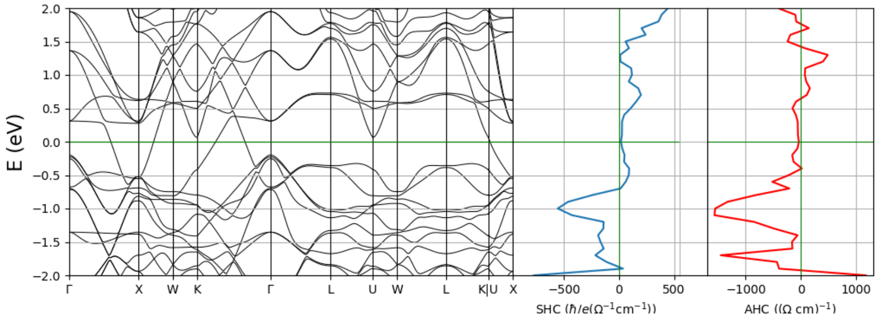


FIG. 17: The electronic band structures and corresponding SHC, AHC for $Co_2NbGa$

### 18. $Co_2NbSn$

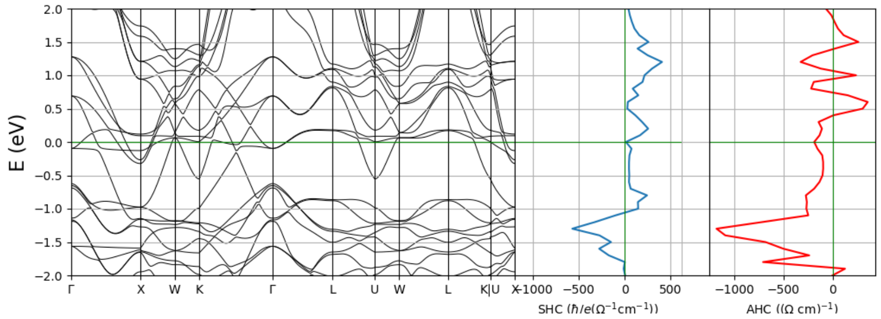


FIG. 18: The electronic band structures and corresponding SHC, AHC for $Co_2NbSn$

### 19. $Co_2MnSb$

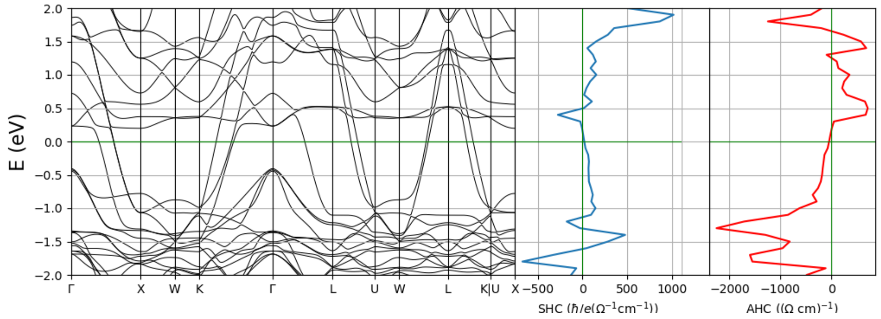


FIG. 19: The electronic band structures and corresponding SHC, AHC for $Co_2MnSb$

### 20. $Co_2ScSn$

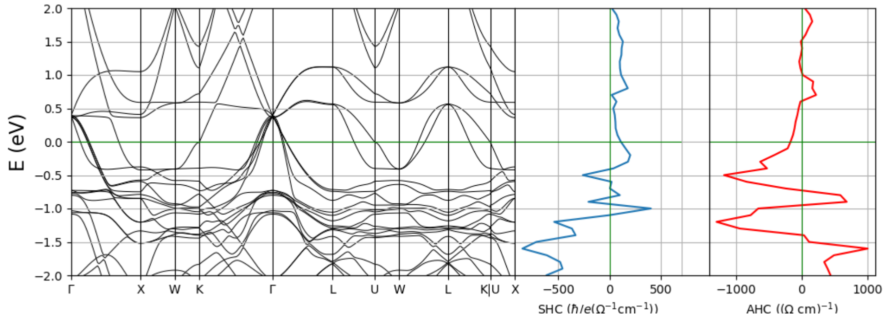


FIG. 20: The electronic band structures and corresponding SHC, AHC for $Co_2ScSn$

### 21. $Co_2FeSi$

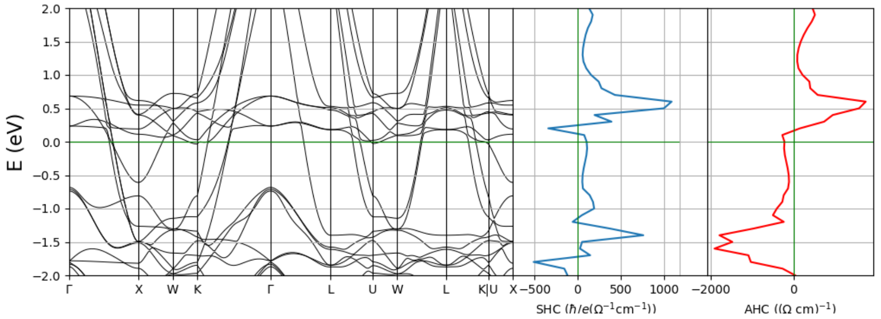


FIG. 21: The electronic band structures and corresponding SHC, AHC for $Co_2FeSi$

### 22. $Co_2MnSi$

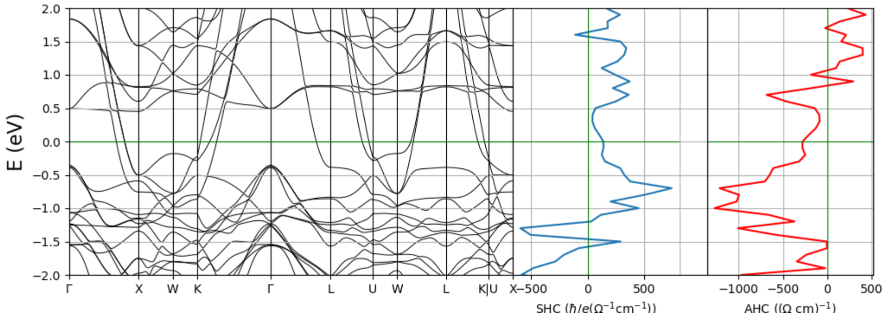


FIG. 22: The electronic band structures and corresponding SHC, AHC for $Co_2MnSi$

### 23. $Co_2VSi$

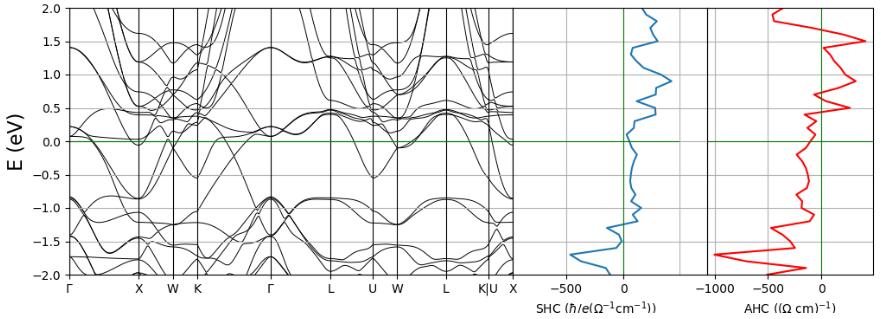


FIG. 23: The electronic band structures and corresponding SHC, AHC for $Co_2VSi$

### 24. $Co_2MnSn$

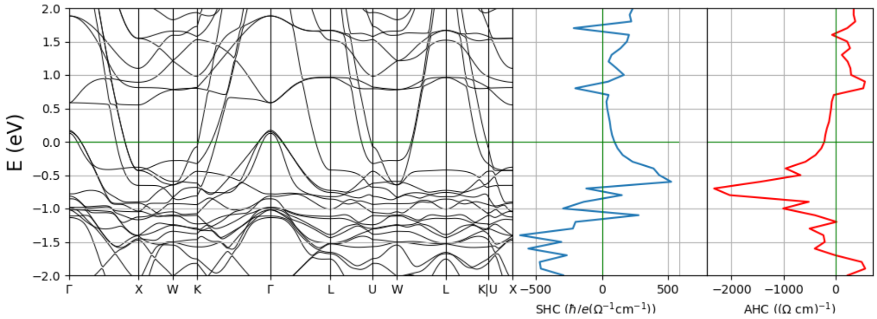


FIG. 24: The electronic band structures and corresponding SHC, AHC for $Co_2MnSn$

### 25. $Co_2TiAl$

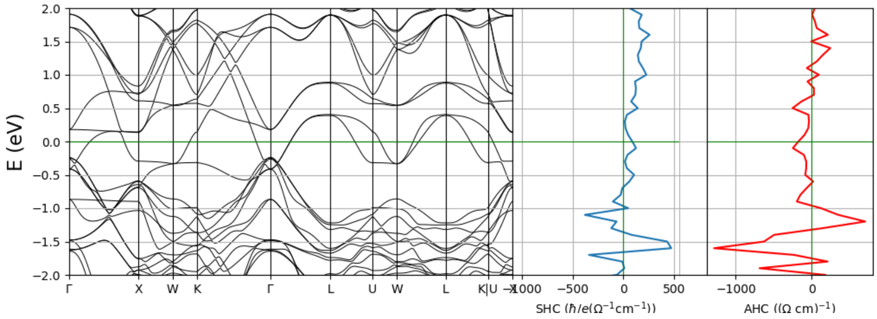


FIG. 25: The electronic band structures and corresponding SHC, AHC for $Co_2TiAl$

### 26. $Co_2TiGa$

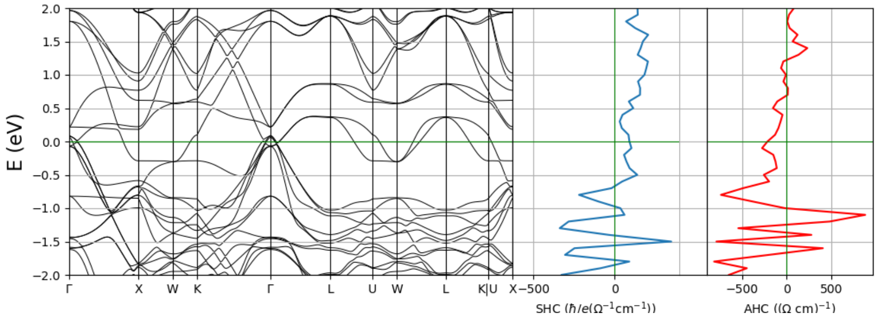


FIG. 26: The electronic band structures and corresponding SHC, AHC for $Co_2TiGa$

### 27. $Co_2TiGe$

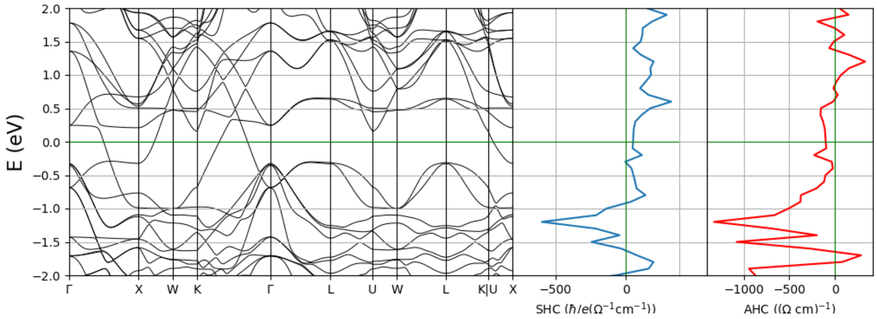


FIG. 27: The electronic band structures and corresponding SHC, AHC for $Co_2TiGe$

### 28. $Co_2TiSi$

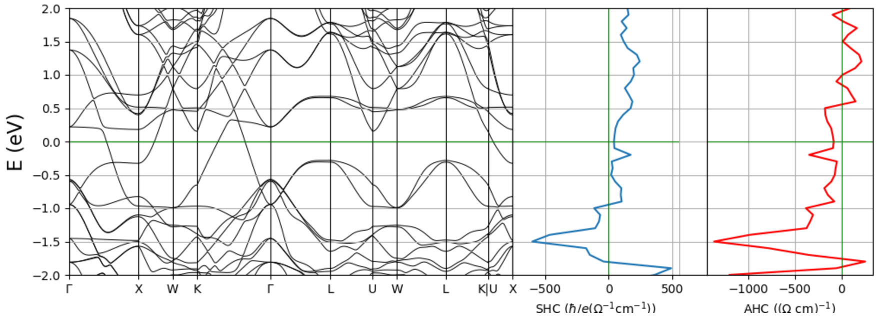


FIG. 28: The electronic band structures and corresponding SHC, AHC for $Co_2TiSi$

### 29. $Co_2TiSn$

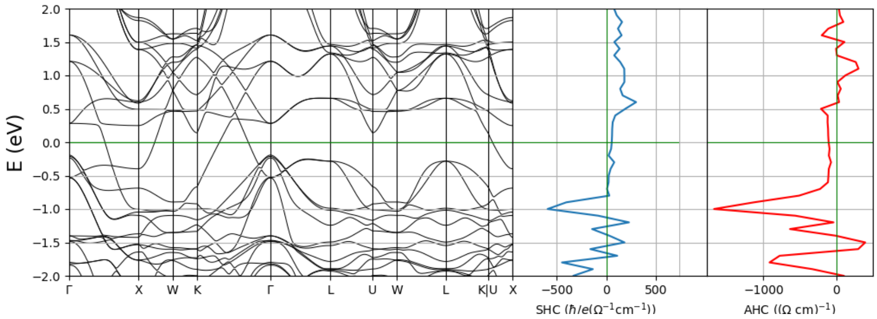


FIG. 29: The electronic band structures and corresponding SHC, AHC for $Co_2TiSn$

### 30. $Co_2VAl$

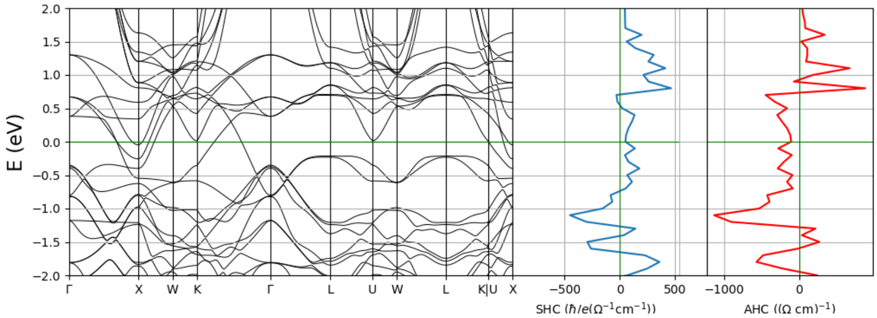


FIG. 30: The electronic band structures and corresponding SHC, AHC for $Co_2VAl$

### 31. $Co_2VGa$

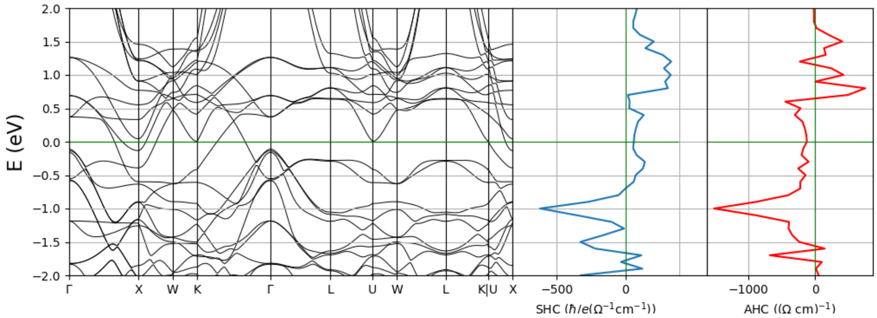


FIG. 31: The electronic band structures and corresponding SHC, AHC for $Co_2VGa$

### 32. $Co_2VSn$

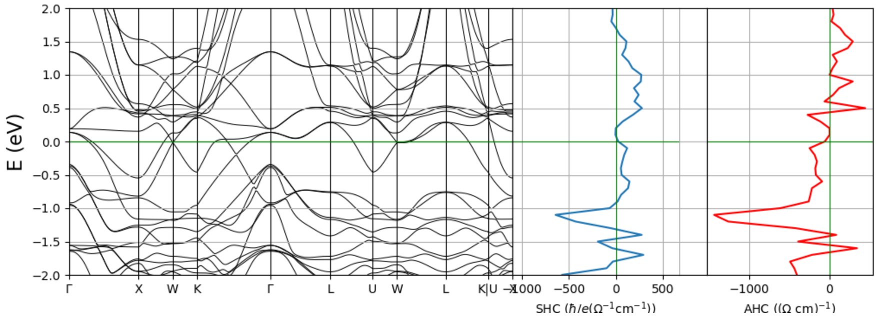


FIG. 32: The electronic band structures and corresponding SHC, AHC for $Co_2VSn$

### 33. $Co_2ZrAl$

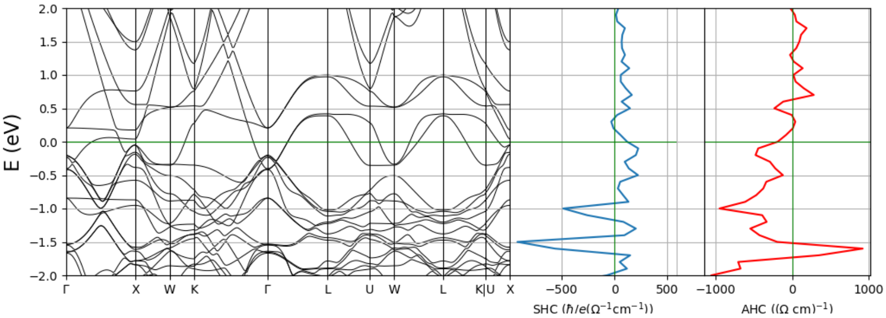


FIG. 33: The electronic band structures and corresponding SHC, AHC for $Co_2ZrAl$

### 34. $Co_2ZrSn$

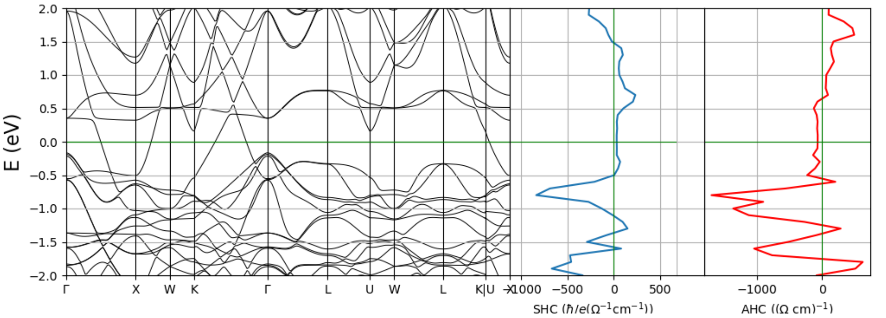


FIG. 34: The electronic band structures and corresponding SHC, AHC for $Co_2ZrSn$

### 35. $Cu_2CoSn$

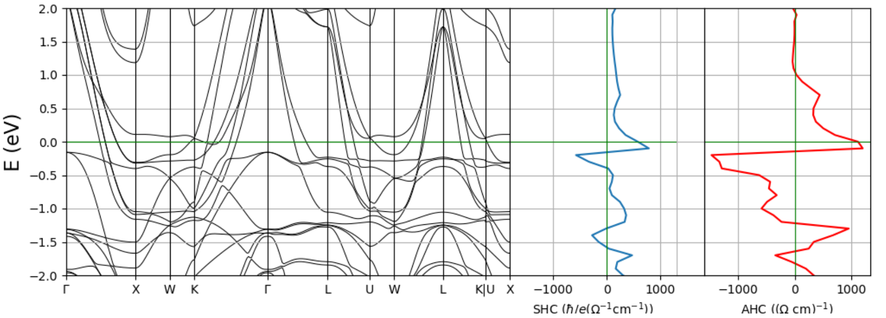


FIG. 35: The electronic band structures and corresponding SHC, AHC for $Cu_2CoSn$

### 36. $Cu_2CrAl$

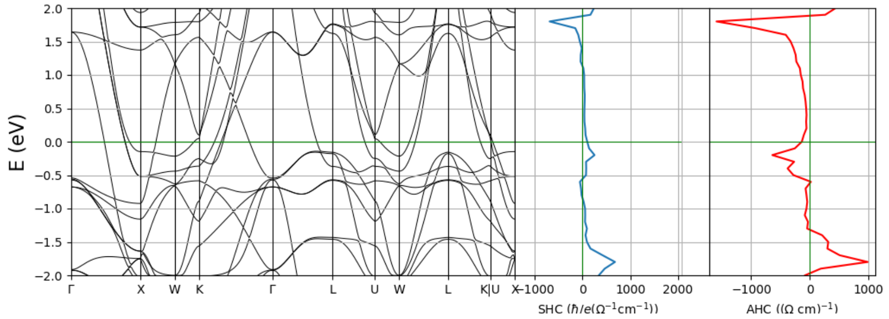


FIG. 36: The electronic band structures and corresponding SHC, AHC for $Cu_2CrAl$

### 37. $Cu_2FeSn$

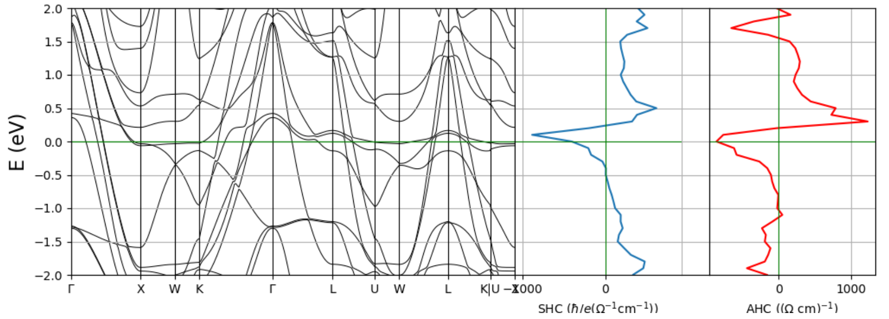


FIG. 37: The electronic band structures and corresponding SHC, AHC for $Cu_2FeSn$

### 38. $Cu_2MnAl$

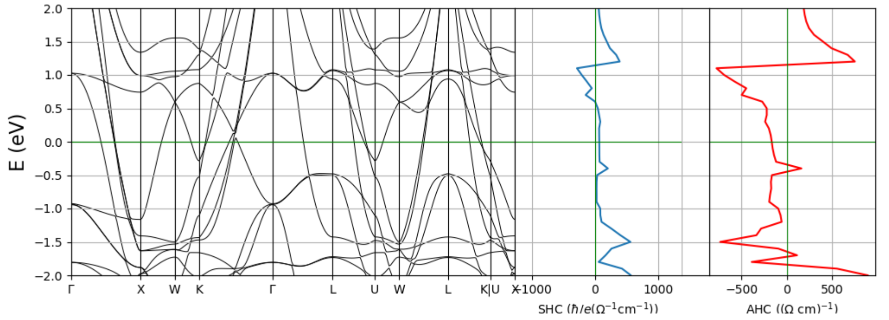


FIG. 38: The electronic band structures and corresponding SHC, AHC for $Cu_2MnAl$

### 39. $Cu_2MnIn$

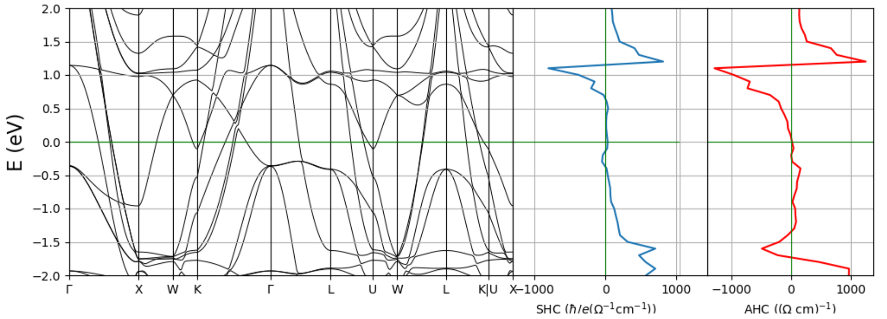


FIG. 39: The electronic band structures and corresponding SHC, AHC for $Cu_2MnIn$

### 40. $Cu_2MnSn$

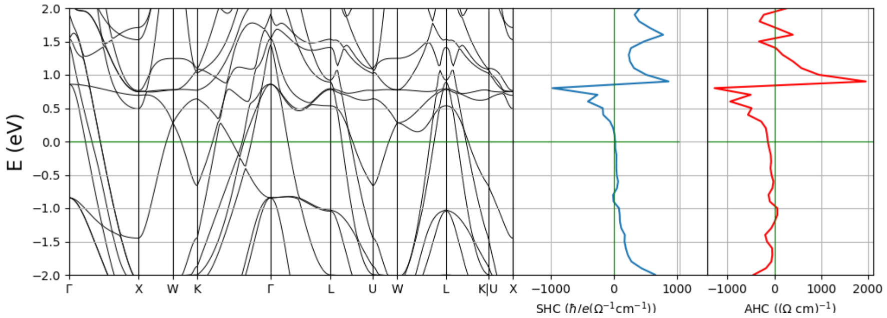


FIG. 40: The electronic band structures and corresponding SHC, AHC for $Cu_2MnSn$

### 41. $Cu_2MnSb$

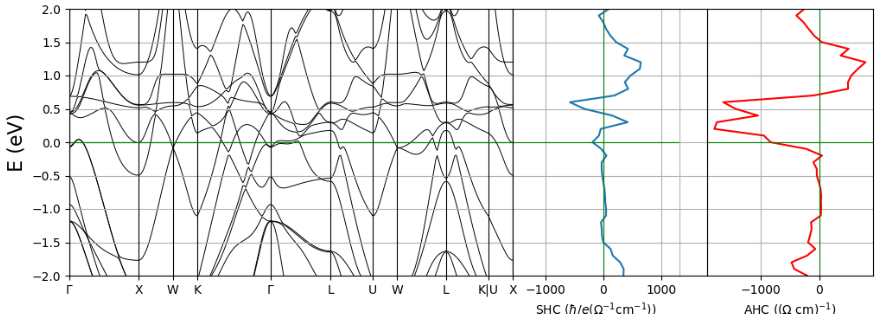


FIG. 41: The electronic band structures and corresponding SHC, AHC for $Cu_2MnSb$

### 42. $Fe_2MoAl$

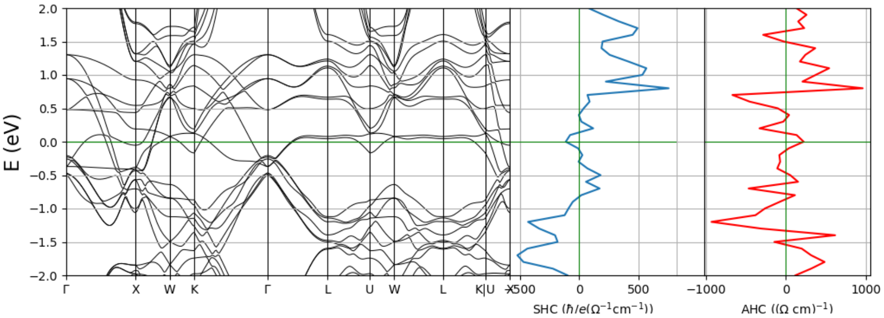


FIG. 42: The electronic band structures and corresponding SHC, AHC for $Fe_2MoAl$

### 43. $Fe_2CrAl$

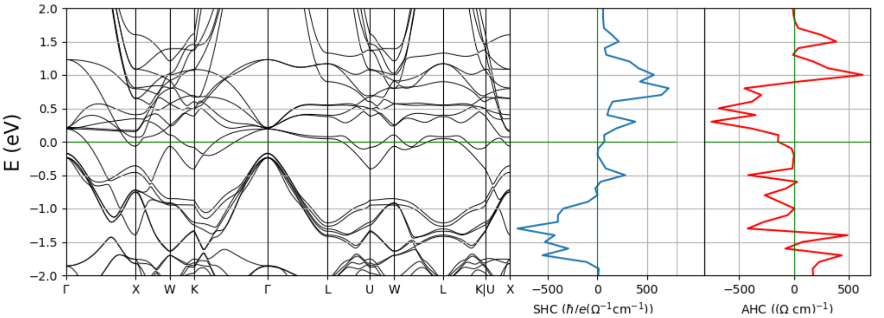


FIG. 43: The electronic band structures and corresponding SHC, AHC for $Fe_2CrAl$

### 44. $Fe_2CoGa$

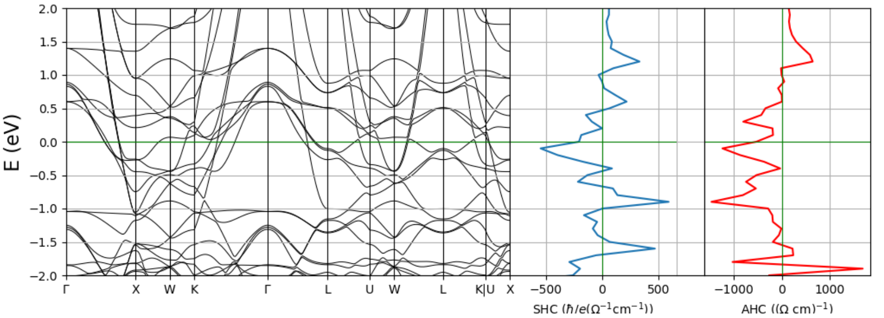


FIG. 44: The electronic band structures and corresponding SHC, AHC for $Fe_2GaCo$

### 45. $Fe_2TiGa$

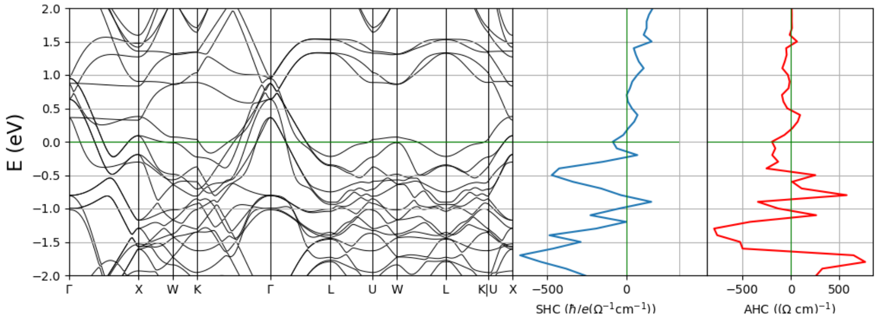


FIG. 45: The electronic band structures and corresponding SHC, AHC for $Fe_2TiGa$

### 46. $Fe_2CoGe$

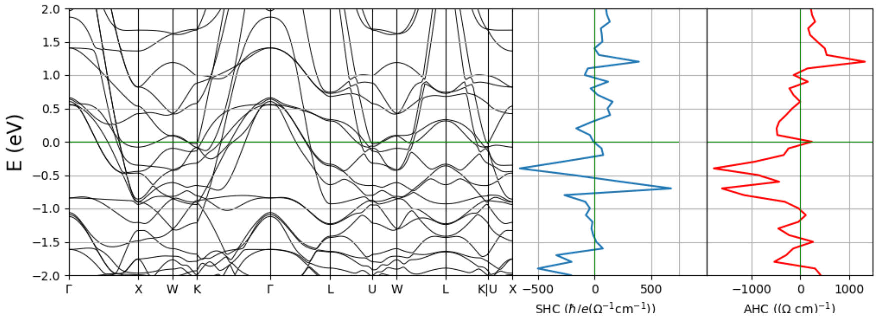


FIG. 46: The electronic band structures and corresponding SHC, AHC for $Fe_2CoGe$

### 47. $Fe_2MnAl$

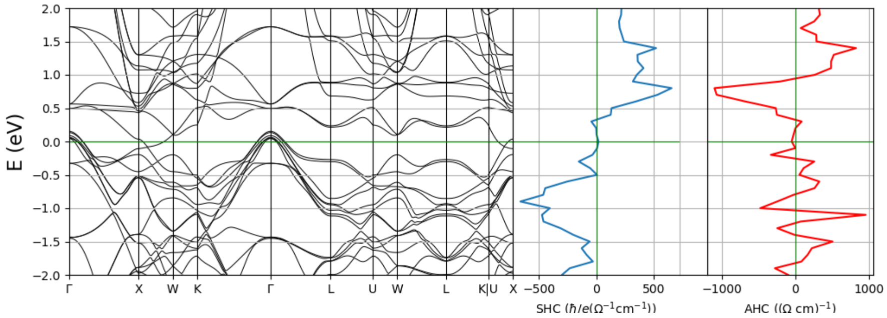


FIG. 47: The electronic band structures and corresponding SHC, AHC for $Fe_2MnAl$

### 48. $Fe_2NiAl$

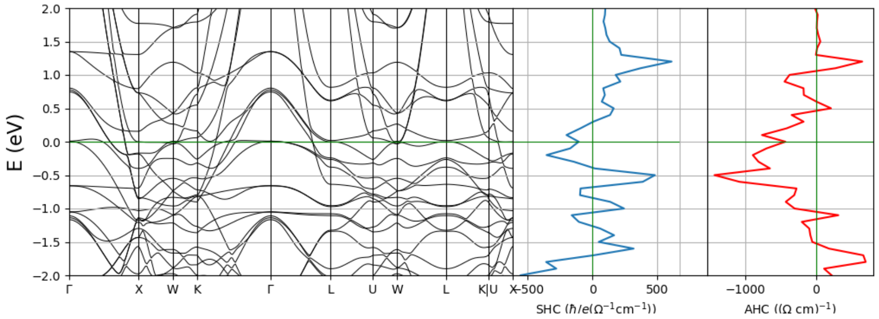


FIG. 48: The electronic band structures and corresponding SHC, AHC for $Fe_2NiAl$

### 49. $Fe_2NiGa$

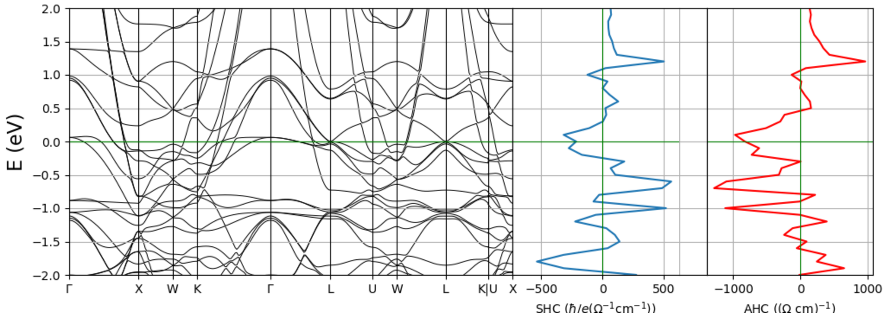


FIG. 49: The electronic band structures and corresponding SHC, AHC for $Fe_2NiGa$

### 50. $Fe_2MnSi$

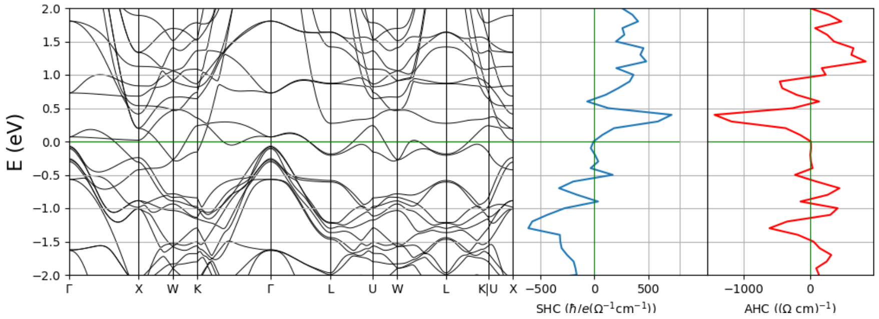


FIG. 50: The electronic band structures and corresponding SHC, AHC for $Fe_2MnSi$

### 51. $Fe_2VSi$

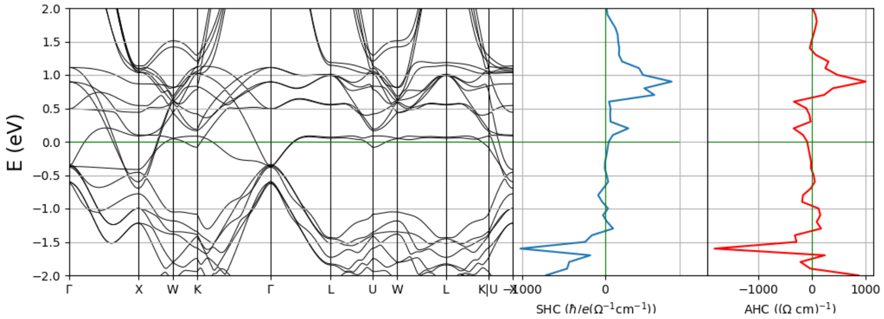


FIG. 51: The electronic band structures and corresponding SHC, AHC for $Fe_2VSi$

### 52. $Fe_2VSn$

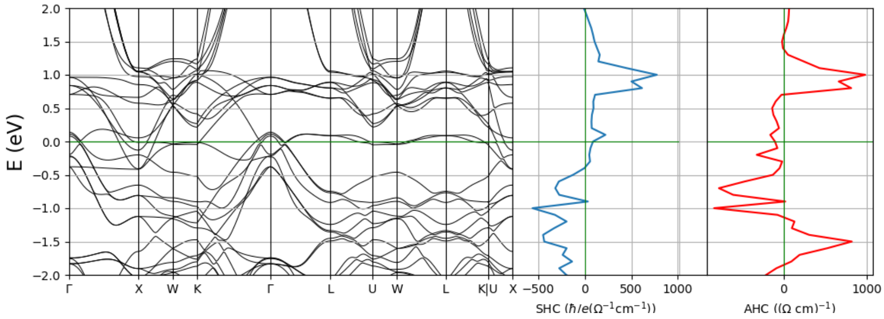


FIG. 52: The electronic band structures and corresponding SHC, AHC for $Fe_2VSn$

### 53. $Fe_2TiAl$

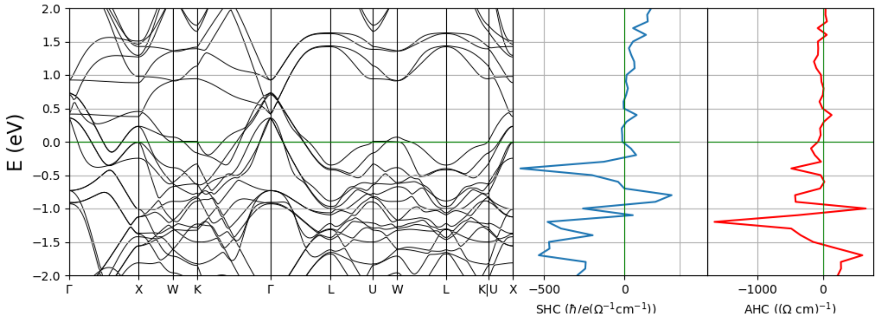


FIG. 53: The electronic band structures and corresponding SHC, AHC for $Fe_2TiAl$

## 54. $Mn_2VAl$

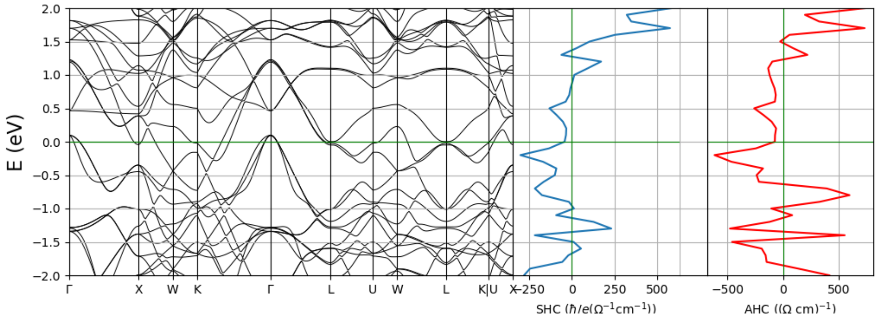


FIG. 54: The electronic band structures and corresponding SHC, AHC for $Mn_2VAl$

## 55. $Ni_2CrAl$

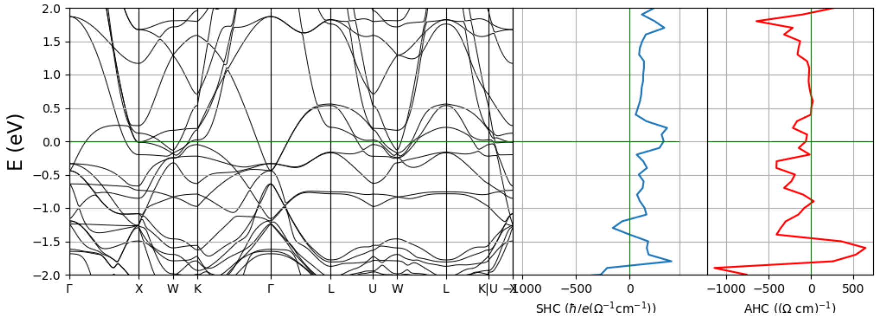


FIG. 55: The electronic band structures and corresponding SHC, AHC for $Ni_2CrAl$

## 56. $Ni_2MnAl$

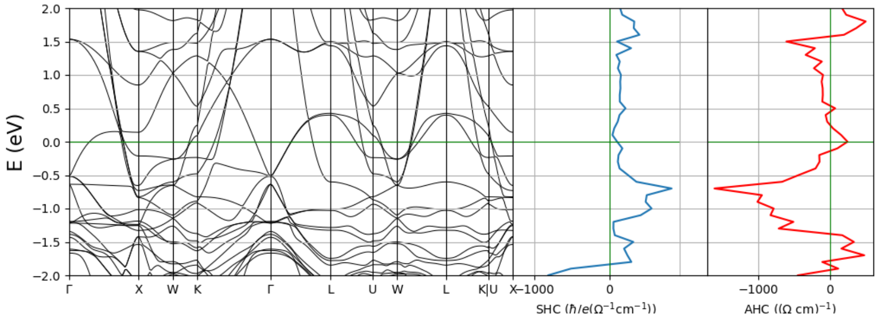


FIG. 56: The electronic band structures and corresponding SHC, AHC for $Ni_2MnAl$

### 57. $Ni_2MnGa$

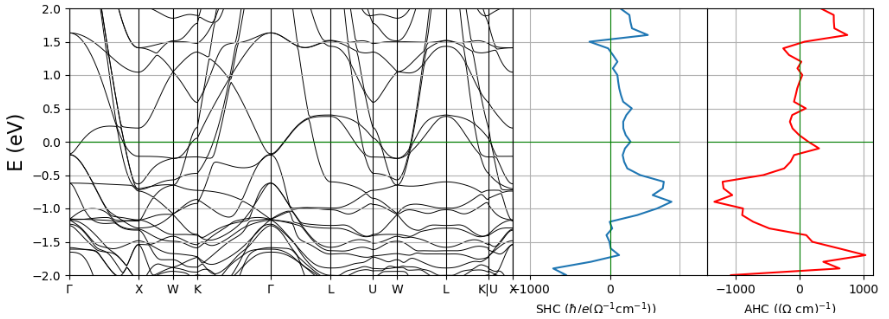


FIG. 57: The electronic band structures and corresponding SHC, AHC for $Ni_2MnGa$

### 58. $Ni_2MnGe$

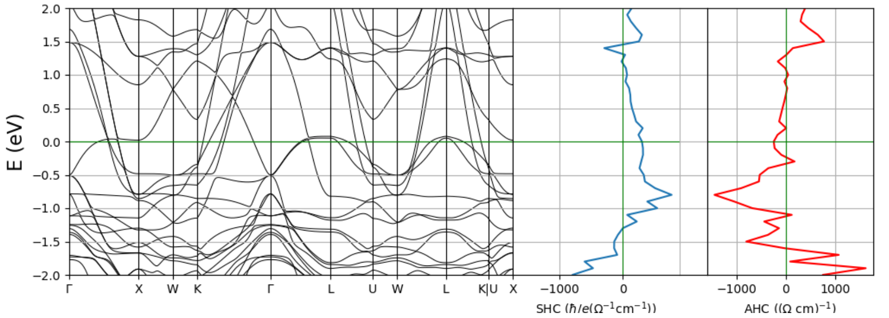


FIG. 58: The electronic band structures and corresponding SHC, AHC for $Ni_2MnGe$

### 59. $Ni_2MnIn$

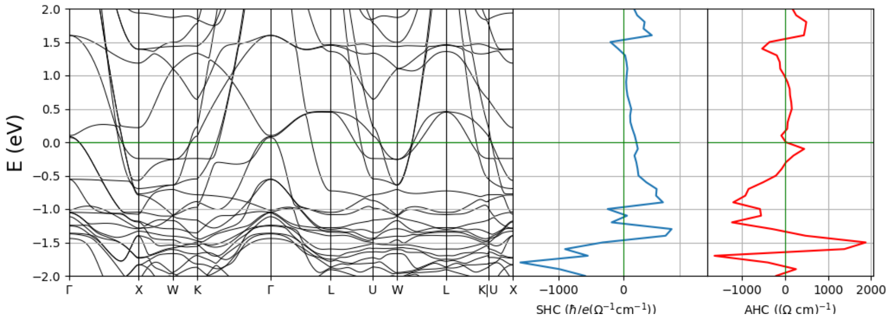


FIG. 59: The electronic band structures and corresponding SHC, AHC for $Ni_2MnIn$

### 60. $Ni_2MnSb$

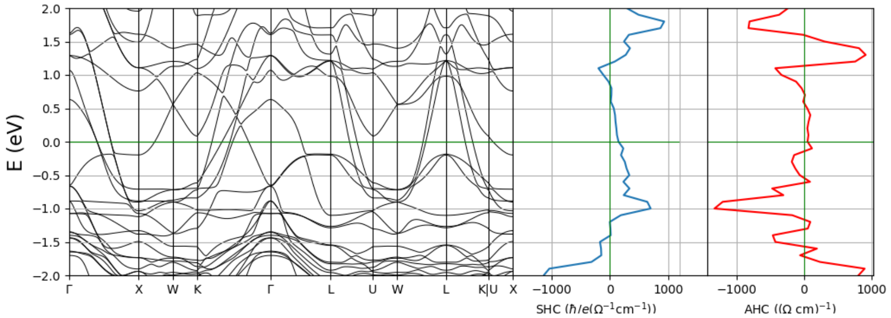


FIG. 60: The electronic band structures and corresponding SHC, AHC for $Ni_2MnSb$

### 61. $Ni_2MnSn$

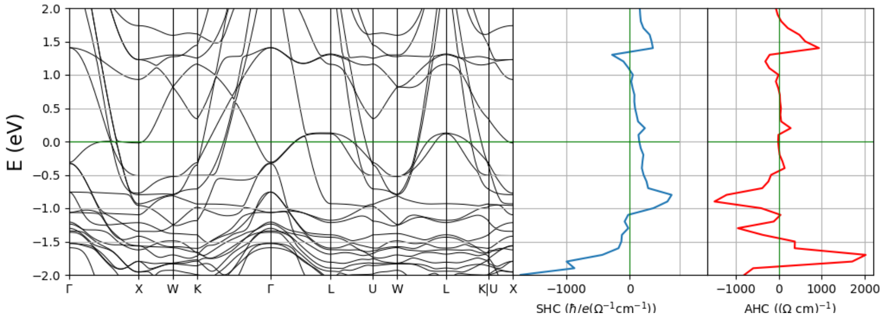


FIG. 61: The electronic band structures and corresponding SHC, AHC for $Ni_2MnSn$

### 62. $Pd_2MnAs$

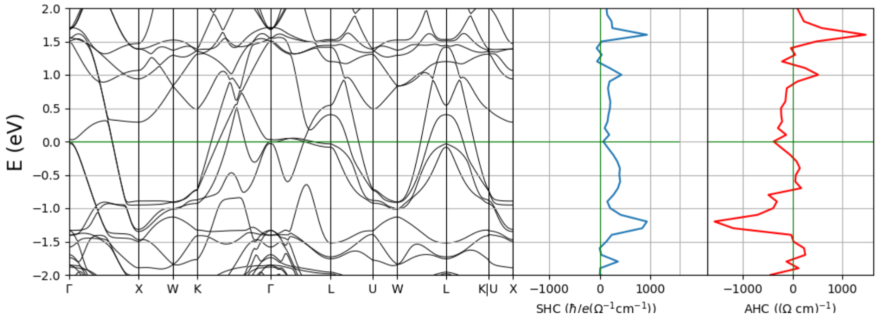


FIG. 62: The electronic band structures and corresponding SHC, AHC for $Pd_2MnAs$

### 63. $Pd_2MnIn$

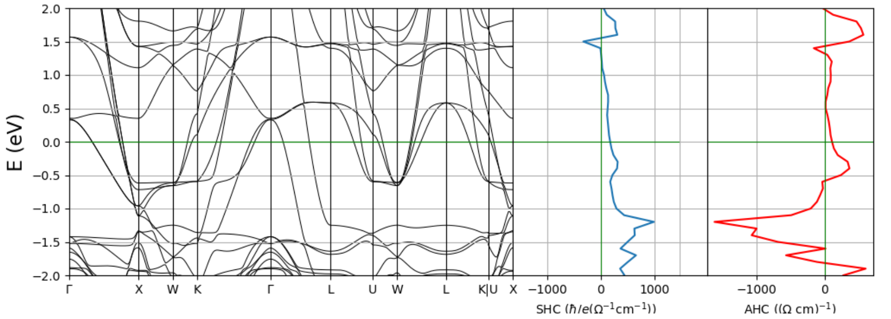


FIG. 63: The electronic band structures and corresponding SHC, AHC for $Pd_2MnIn$

### 64. $Pd_2MnSb$

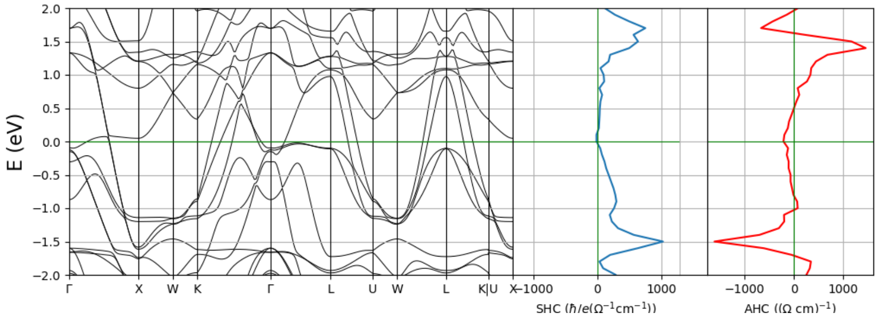


FIG. 64: The electronic band structures and corresponding SHC, AHC for $Pd_2MnSb$

### 65. $Pd_2MnSn$

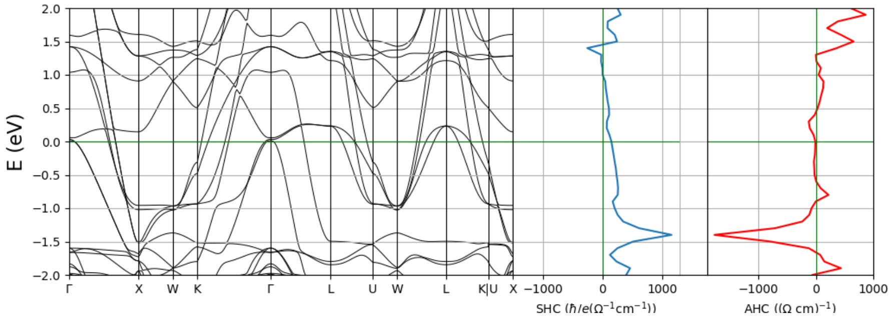


FIG. 65: The electronic band structures and corresponding SHC, AHC for $Pd_2MnSn$

### 66. $Rh_2MnAl$

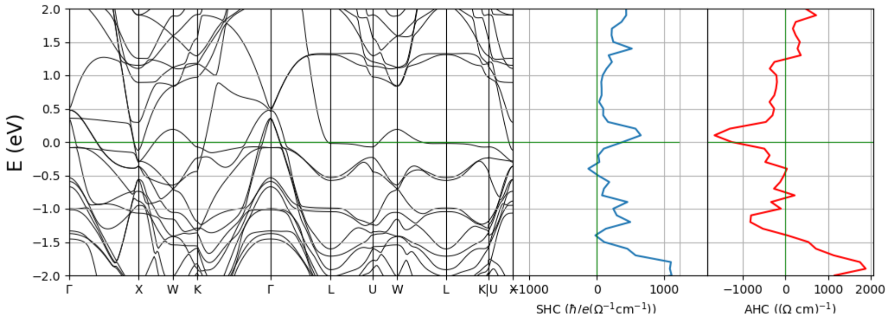


FIG. 66: The electronic band structures and corresponding SHC, AHC for $Rh_2MnAl$

### 67. $Rh_2MnGe$

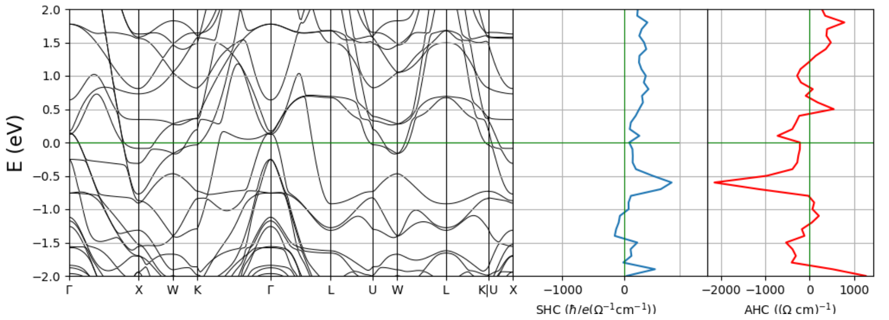


FIG. 67: The electronic band structures and corresponding SHC, AHC for $Rh_2MnGe$

### 68. $Rh_2MnPb$

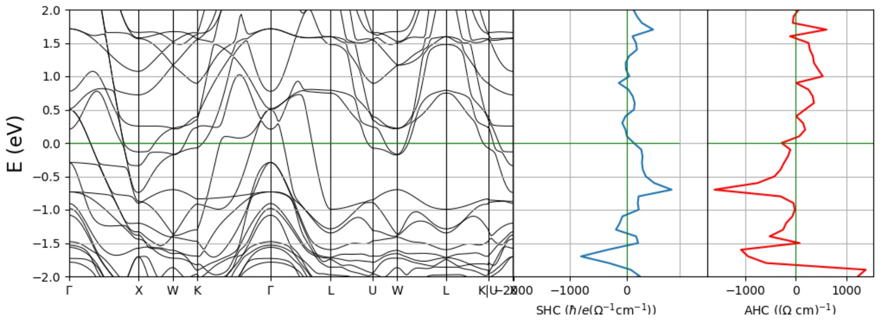


FIG. 68: The electronic band structures and corresponding SHC, AHC for $Rh_2MnPb$

### 69. $Rh_2MnSn$

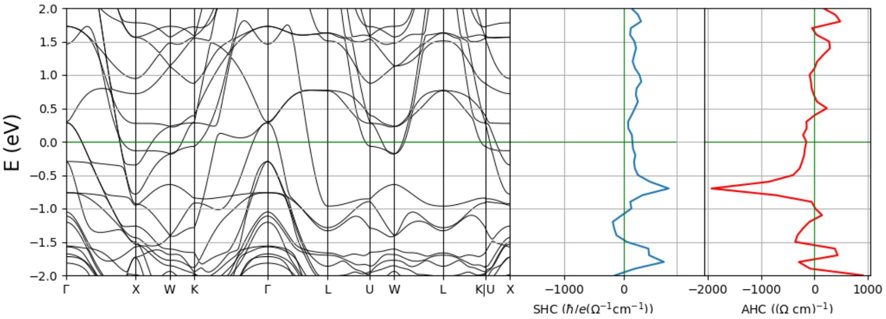


FIG. 69: The electronic band structures and corresponding SHC, AHC for $Rh_2MnSn$

### 70. $Rh_2NiSn$

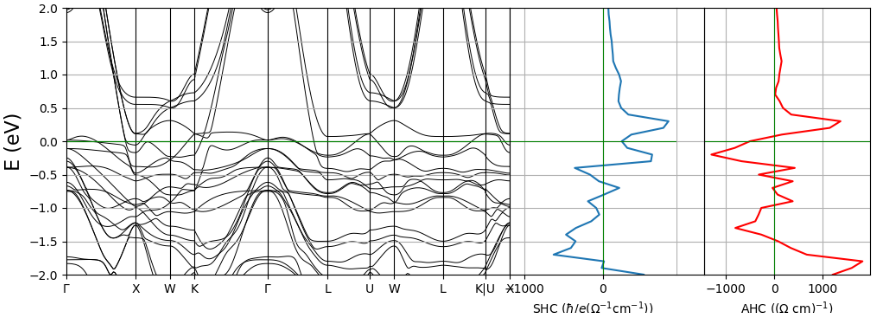


FIG. 70: The electronic band structures and corresponding SHC, AHC for $Rh_2NiSn$

### 71. $Ru_2FeSi$

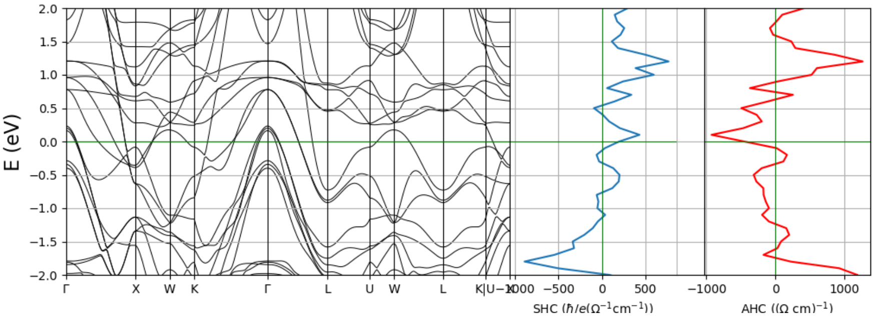


FIG. 71: The electronic band structures and corresponding SHC, AHC for $Ru_2FeSi$

### 72. $Ru_2FeSn$

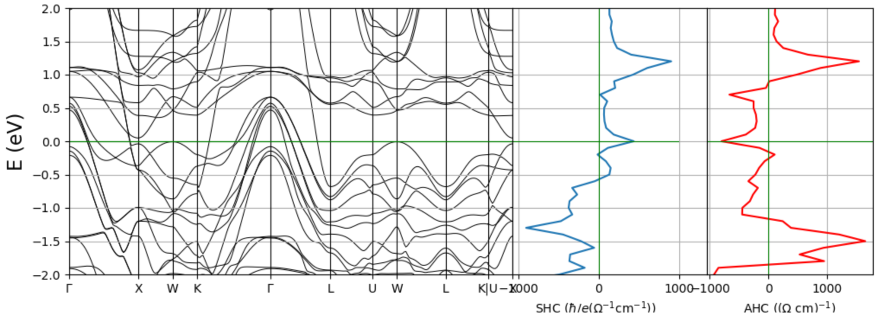


FIG. 72: The electronic band structures and corresponding SHC, AHC for $Ru_2FeSn$

## II. DETAILS FOR NOMAGNETIC FULL HEUSLER MATERIALS

The band structures of nonmagnetic full Heusler materials as well as the corresponding SHC within ±2 eV around the Fermi level are shown in the below.

### 1. $Co_2LiGe$

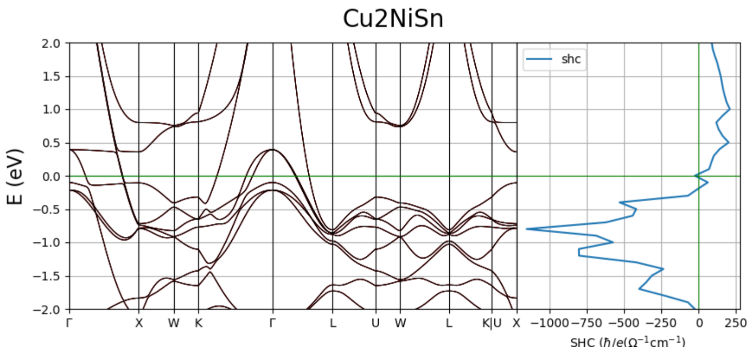


FIG. 73: The electronic band structures and corresponding SHC for $Co_2LiGe$

#### 2. $Co_2TaGa$

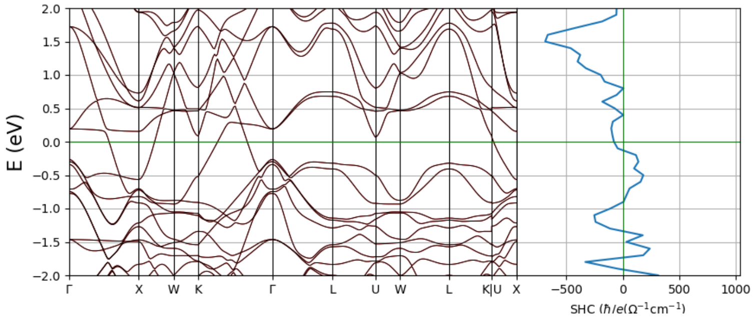


FIG. 74: The electronic band structures and corresponding SHC for $Co_2TaGa$

#### 3. $Co_2ZnGe$

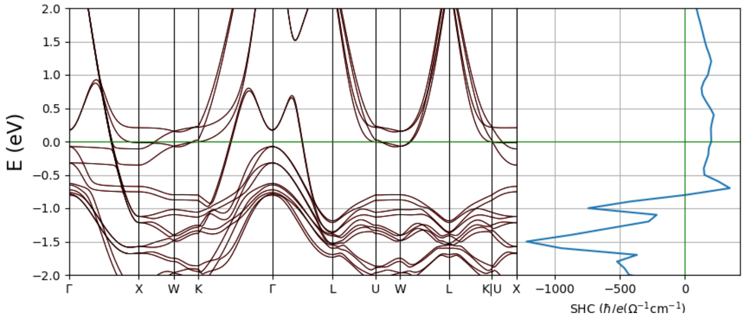


FIG. 75: The electronic band structures and corresponding SHC for $Co_2ZnGe$

#### 4. $Cu_2NiSn$

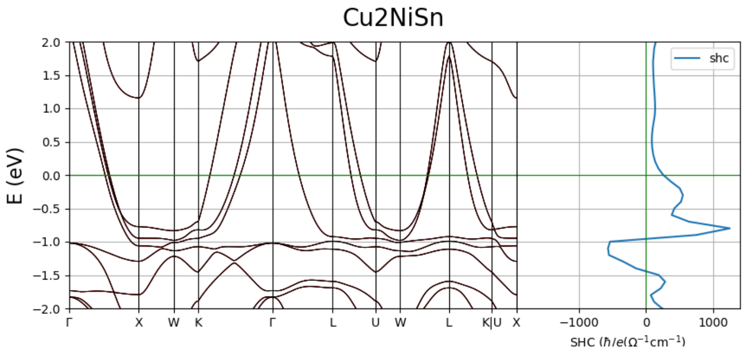


FIG. 76: The electronic band structures and corresponding SHC for $Cu_2NiSn$

### 5. $Fe_2CrGa$

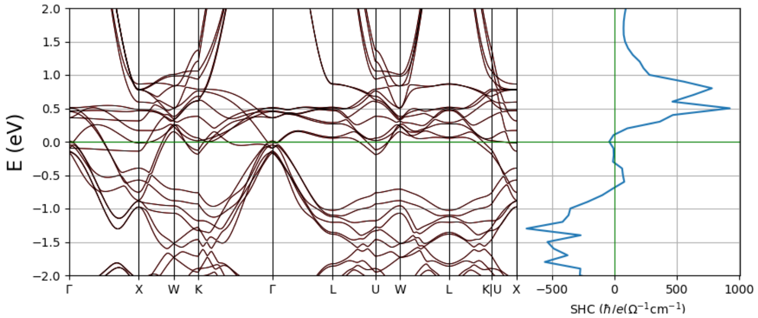


FIG. 77: The electronic band structures and corresponding SHC for $Fe_2CrGa$

### 6. $Fe_2TiSn$

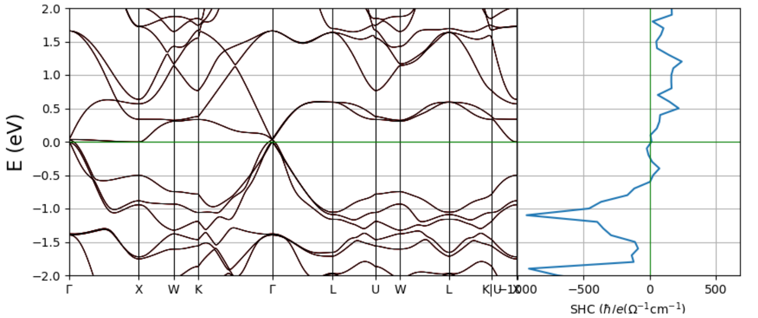


FIG. 78: The electronic band structures and corresponding SHC for $Fe_2TiSn$

### 7. $Fe_2VAl$

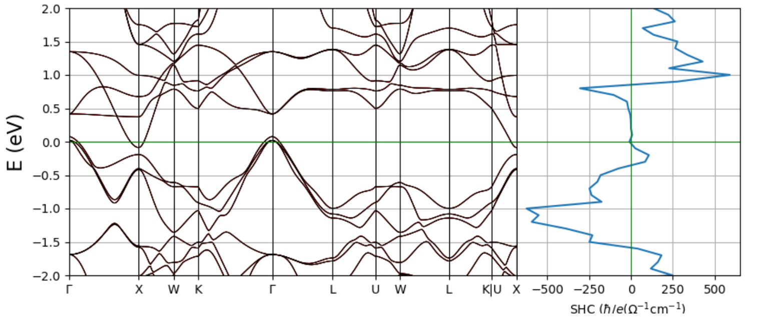


FIG. 79: The electronic band structures and corresponding SHC for $Fe_2VAl$

### 8. $Fe_2VGa$

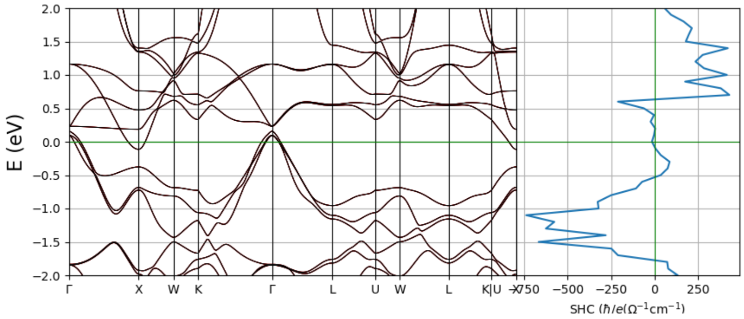


FIG. 80: The electronic band structures and corresponding SHC for $Fe_2VGa$

### 9. $Mn_2VGa$

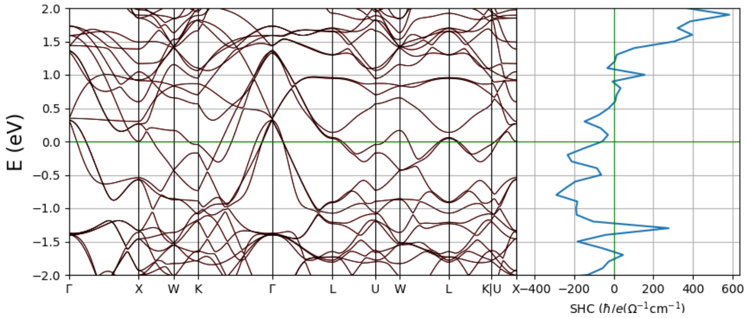


FIG. 81: The electronic band structures and corresponding SHC for $Mn_2VGa$

### 10. $Mn_2WSn$

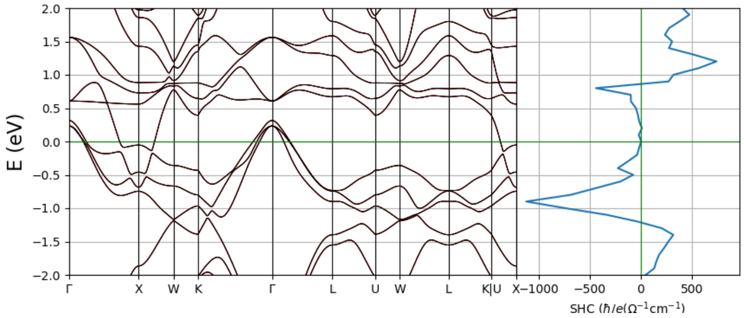


FIG. 82: The electronic band structures and corresponding SHC for $Mn_2WSn$

### 11. $Ni_2ZnGe$

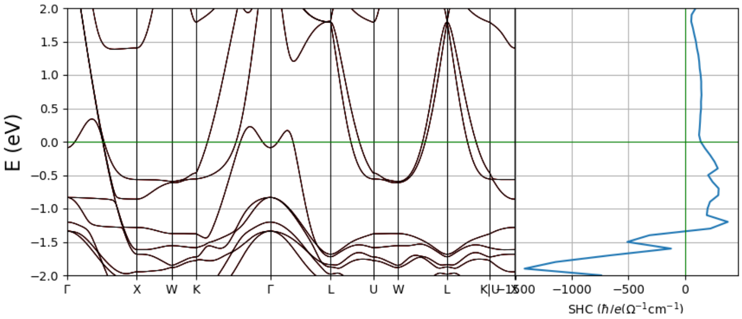


FIG. 83: The electronic band structures and corresponding SHC for $Ni_2ZnGe$

### 12. $Ni_2HfAl$

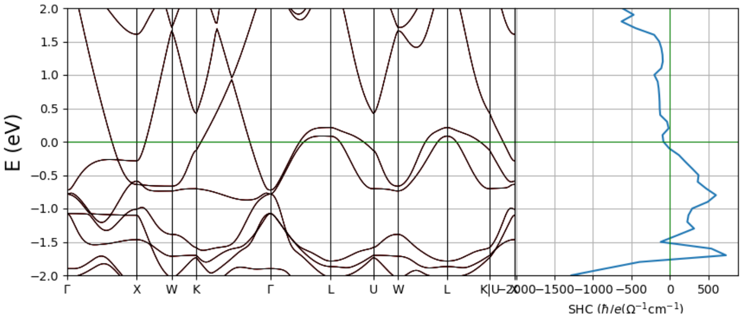


FIG. 84: The electronic band structures and corresponding SHC for $Ni_2HfAl$

### 13. $Ni_2HfGa$

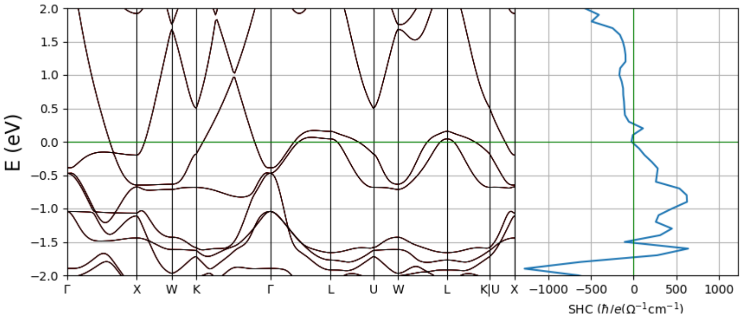


FIG. 85: The electronic band structures and corresponding SHC for $Ni_2HfGa$

### 14. $Ni_2HfIn$

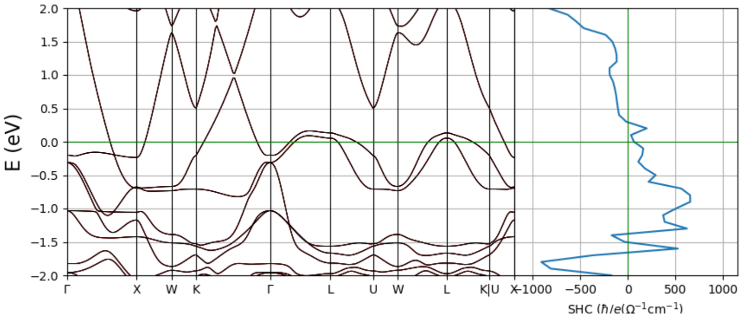


FIG. 86: The electronic band structures and corresponding SHC for $Ni_2HfIn$

### 15. $Ni_2HfSn$

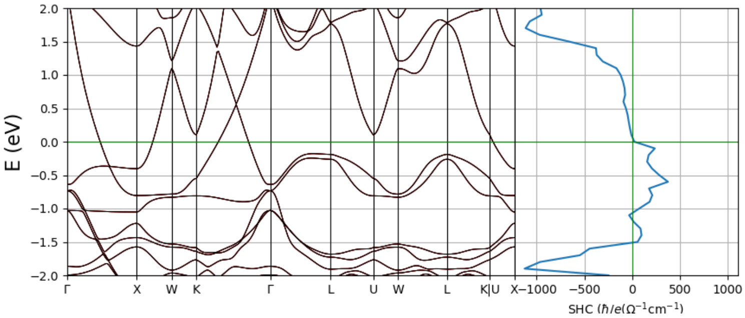


FIG. 87: The electronic band structures and corresponding SHC for $Ni_2HfSn$

### 16. $Ni_2LiGe$

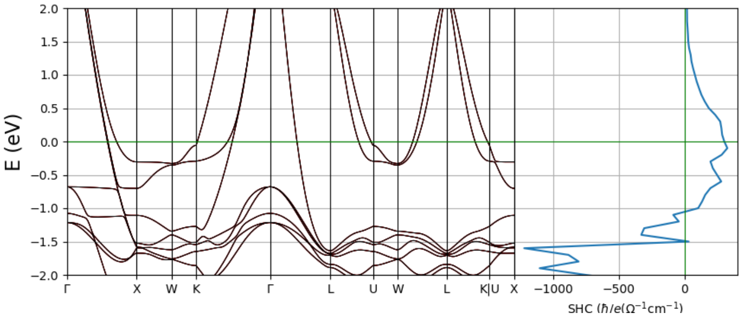


FIG. 88: The electronic band structures and corresponding SHC for $Ni_2LiGe$

### 17. $Ni_2LiSi$

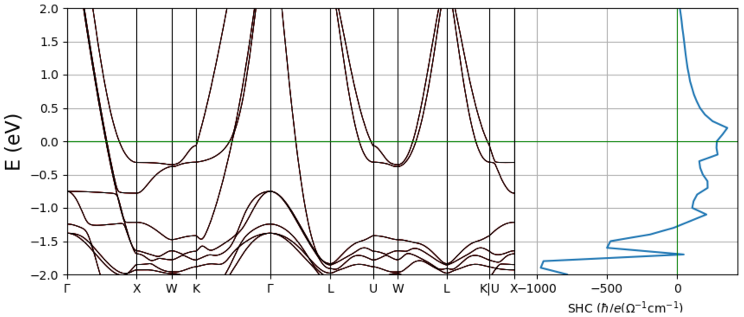


FIG. 89: The electronic band structures and corresponding SHC for $Ni_2LiSi$

### 18. $Ni_2LiSn$

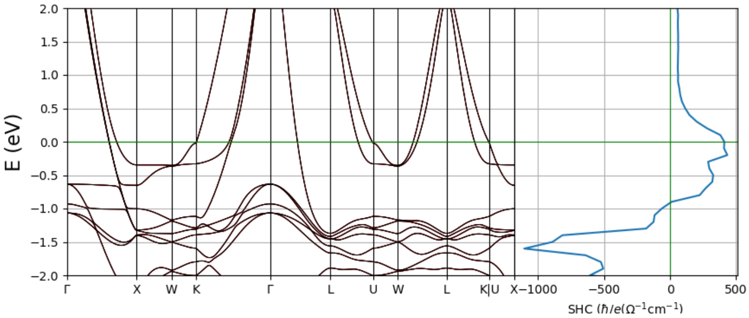


FIG. 90: The electronic band structures and corresponding SHC for $Ni_2LiSn$

### 19. $Ni_2MgIn$

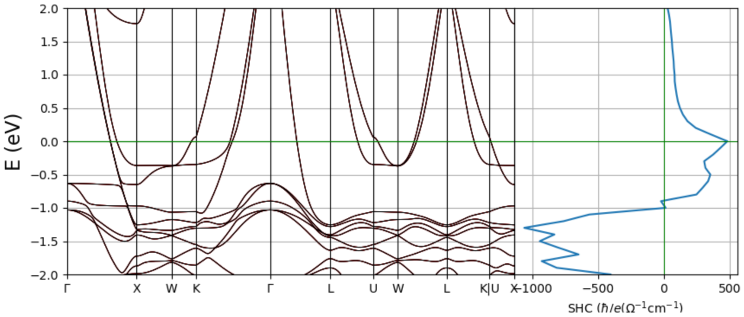


FIG. 91: The electronic band structures and corresponding SHC for $Ni_2MgIn$

### 20. $Ni_2MgSb$

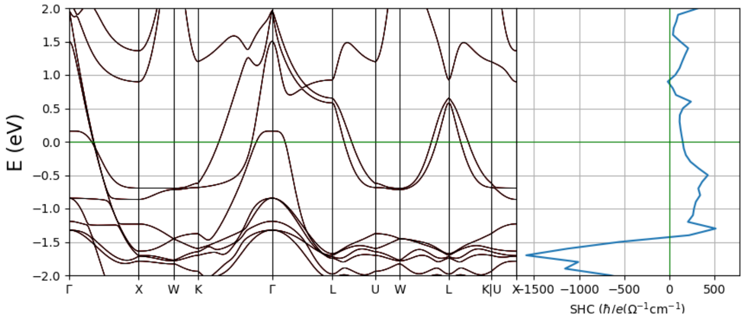


FIG. 92: The electronic band structures and corresponding SHC for $Ni_2MgSb$

### 21. $Ni_2MgSn$

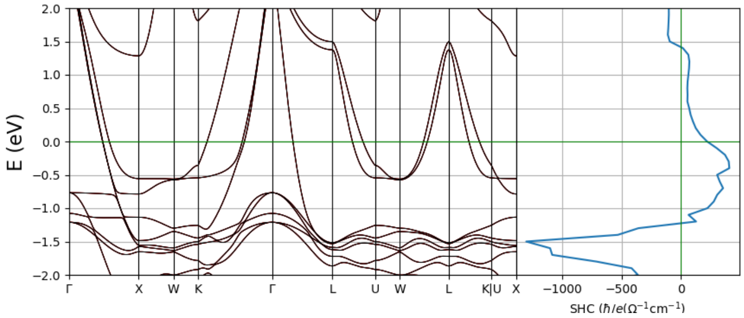


FIG. 93: The electronic band structures and corresponding SHC for $Ni_2MgSn$

### 22. $Ni_2NbAl$

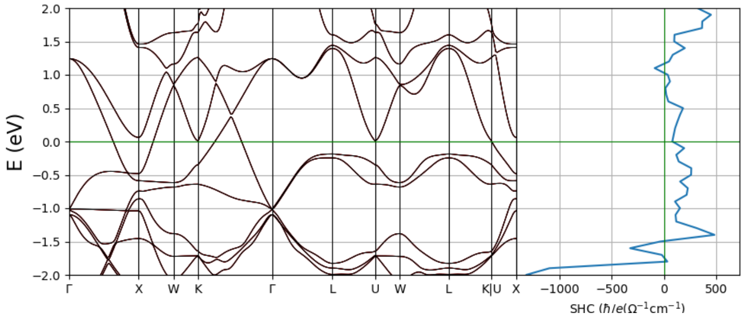


FIG. 94: The electronic band structures and corresponding SHC for $Ni_2NbAl$

### 23. $Ni_2NbGa$

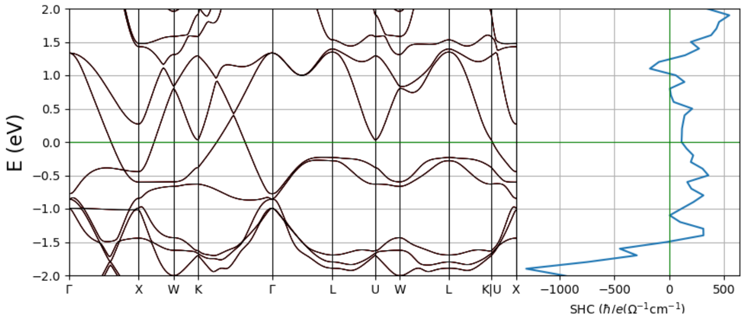


FIG. 95: The electronic band structures and corresponding SHC for $Ni_2NbGa$

### 24. $Ni_2NbSn$

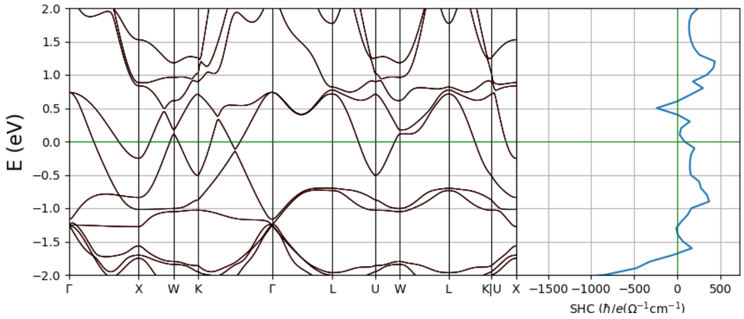


FIG. 96: The electronic band structures and corresponding SHC for $Ni_2NbSn$

### 25. $Ni_2CuSb$

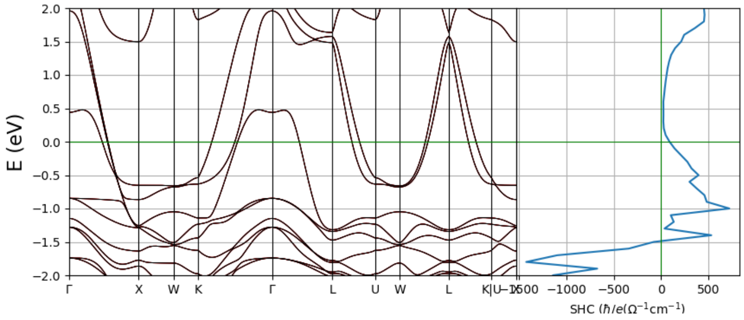


FIG. 97: The electronic band structures and corresponding SHC for $Ni_2CuSb$

### 26. $Ni_2ScAl$

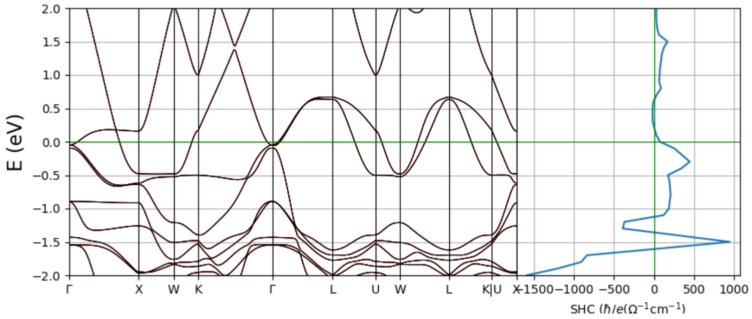


FIG. 98: The electronic band structures and corresponding SHC for $Ni_2ScAl$

### 27. $Ni_2ScGa$

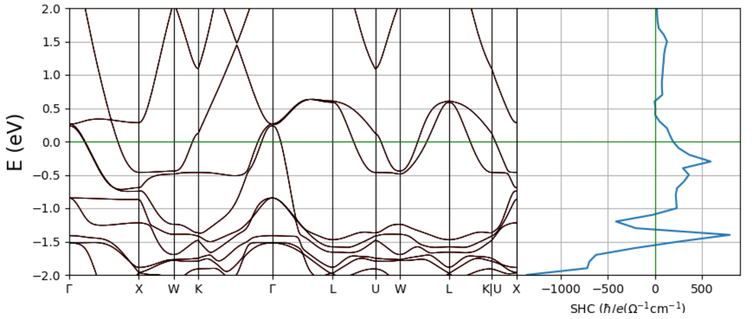


FIG. 99: The electronic band structures and corresponding SHC for $Ni_2ScGa$

### 28. $Ni_2ScIn$

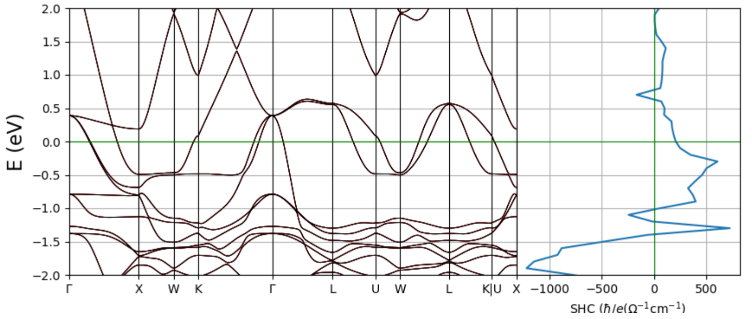


FIG. 100: The electronic band structures and corresponding SHC for $Ni_2ScIn$

## 29. $Ni_2CuSn$

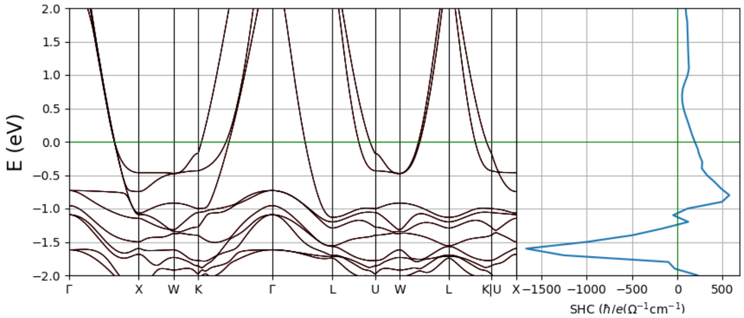


FIG. 101: The electronic band structures and corresponding SHC for $Ni_2CuSn$

## 30. $Ni_2ScSn$

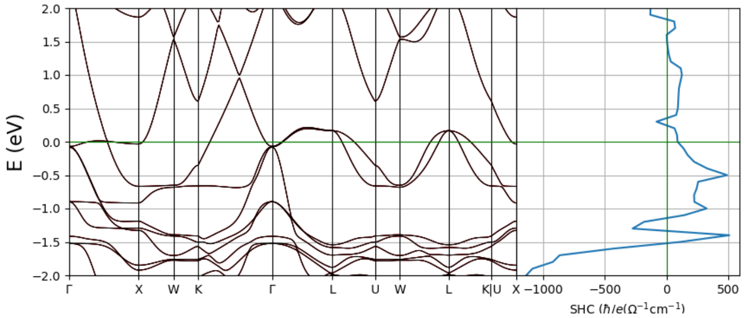


FIG. 102: The electronic band structures and corresponding SHC for $Ni_2ScSn$

## 31. $Ni_2ZrSn$

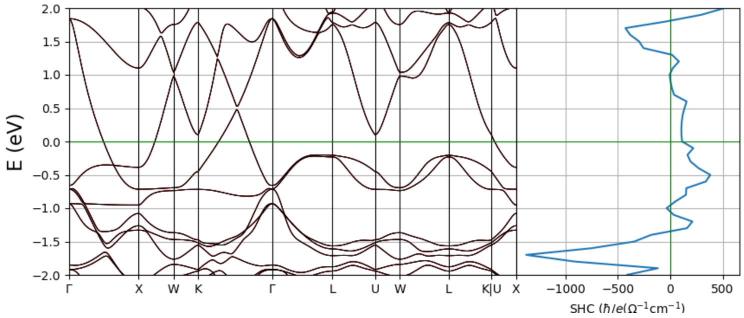


FIG. 103: The electronic band structures and corresponding SHC for $Ni_2ZrSn$

### 32. $Ni_2TaAl$

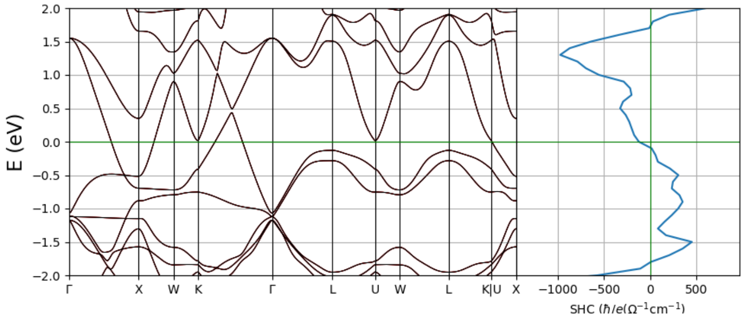


FIG. 104: The electronic band structures and corresponding SHC for $Ni_2TaAl$

### 33. $Ni_2TaGa$

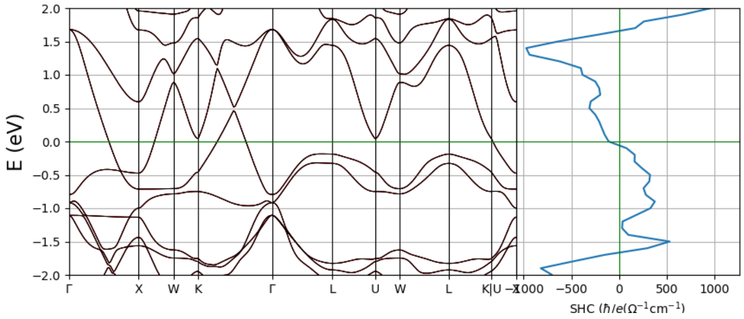


FIG. 105: The electronic band structures and corresponding SHC for $Ni_2TaGa$

### 34. $Ni_2TiAl$

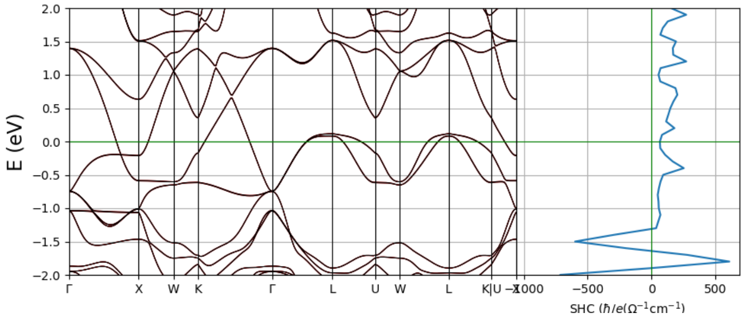


FIG. 106: The electronic band structures and corresponding SHC for $Ni_2TiAl$

### 35. $Ni_2TiGa$

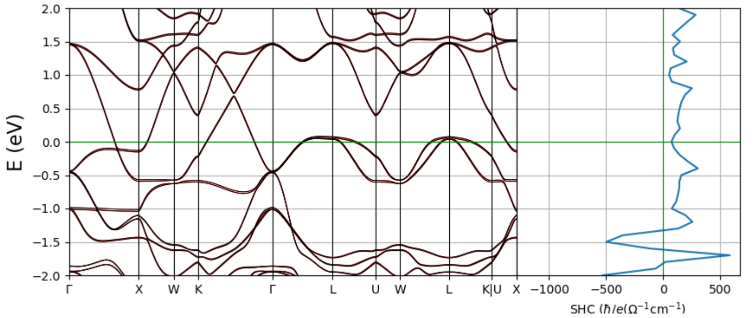


FIG. 107: The electronic band structures and corresponding SHC for $Ni_2TiGa$

### 36. $Ni_2TiIn$

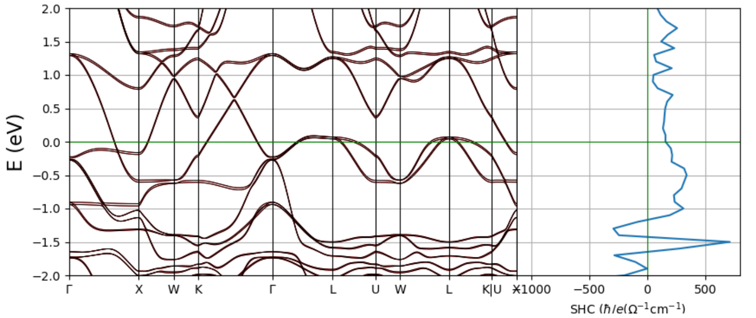


FIG. 108: The electronic band structures and corresponding SHC for $Ni_2TiIn$

### 37. $Ni_2TiSb$

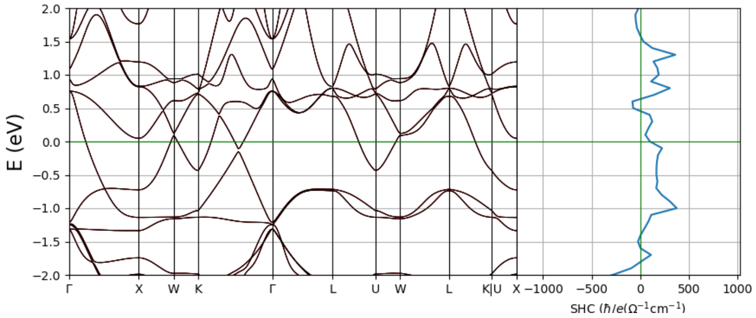


FIG. 109: The electronic band structures and corresponding SHC for $Ni_2TiSb$

### 38. $Ni_2TiSn$

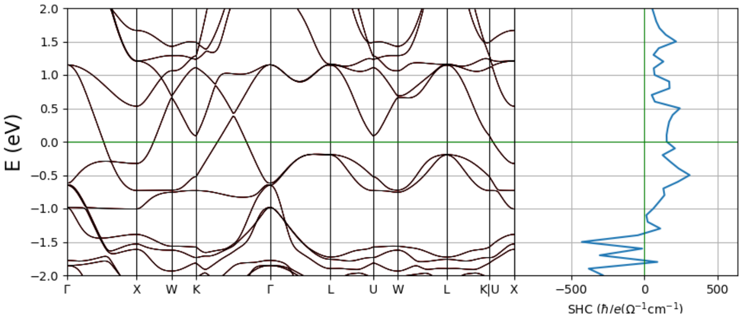


FIG. 110: The electronic band structures and corresponding SHC for $Ni_2TiSn$

### 39. $Ni_2VAl$

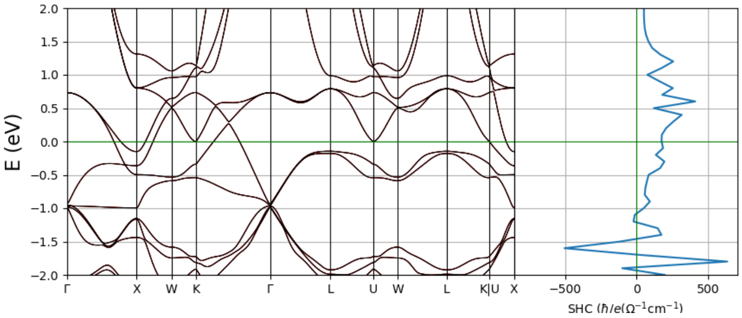


FIG. 111: The electronic band structures and corresponding SHC for $Ni_2VAl$

### 40. $Ni_2VGa$

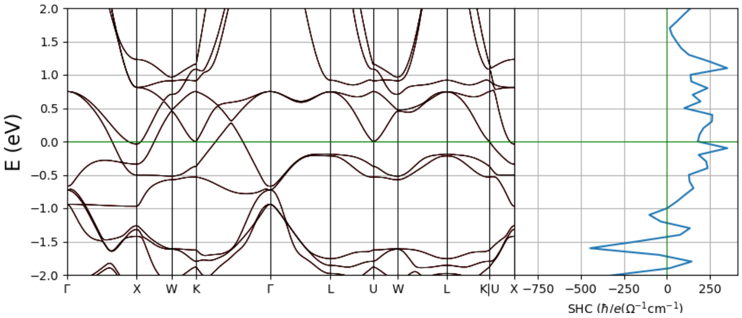


FIG. 112: The electronic band structures and corresponding SHC for $Ni_2VGa$

### 41. $Ni_2VSn$

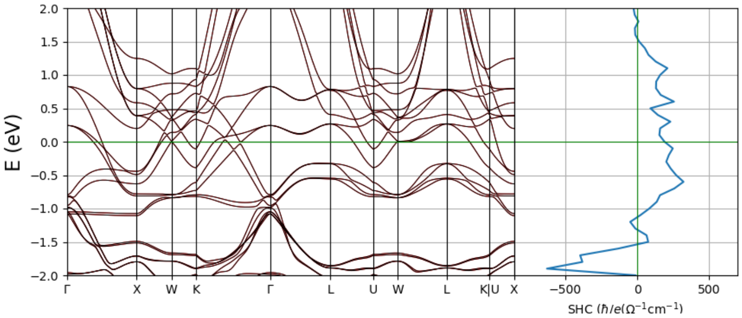


FIG. 113: The electronic band structures and corresponding SHC for $Ni_2VSn$

### 42. $Ni_2YbSn$

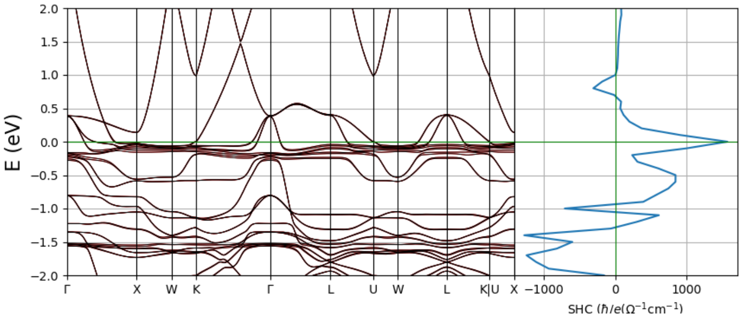


FIG. 114: The electronic band structures and corresponding SHC for $Ni_2YbSn$

### 43. $Ni_2ZrAl$

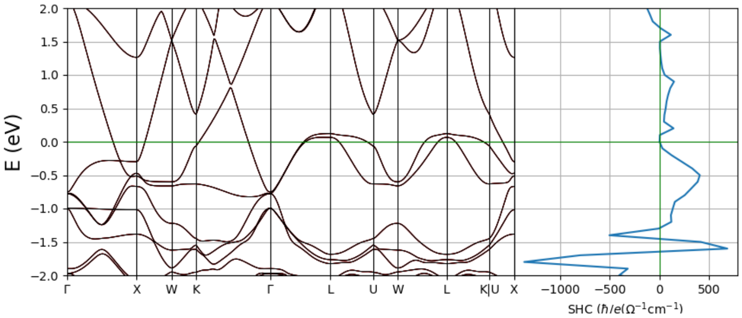


FIG. 115: The electronic band structures and corresponding SHC for $Ni_2ZrAl$

### 44. $Ni_2ZrGa$

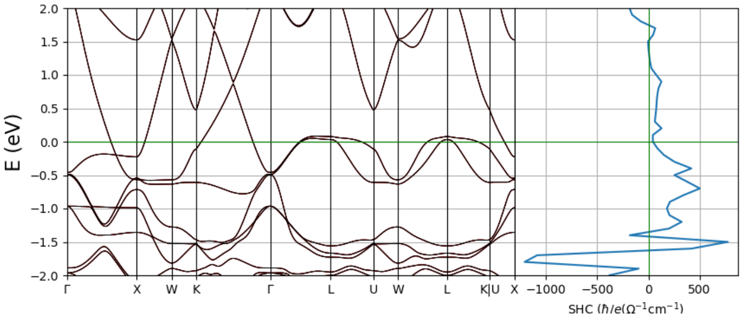


FIG. 116: The electronic band structures and corresponding SHC for $Ni_2ZrGa$

### 45. $Ni_2ZrIn$

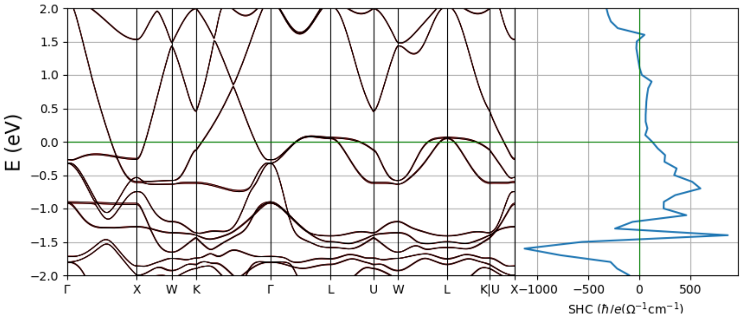


FIG. 117: The electronic band structures and corresponding SHC for $Ni_2ZrIn$

### 46. $Ni_2ZrSb$

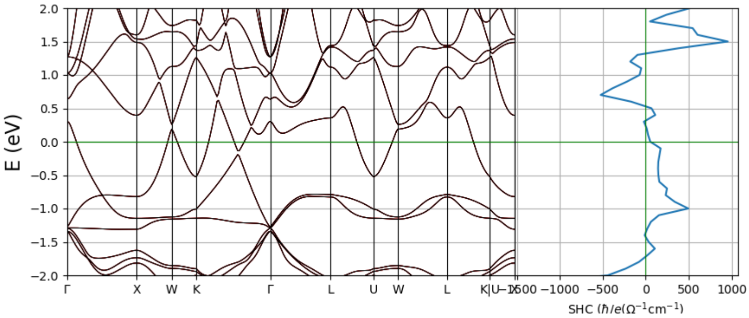


FIG. 118: The electronic band structures and corresponding SHC for $Ni_2ZrSb$

### 47. $Pd_2MnGe$

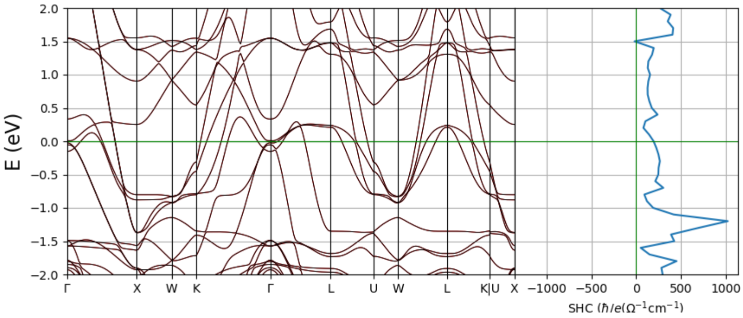


FIG. 119: The electronic band structures and corresponding SHC for $Pd_2MnGe$
